# Supplementary material for: Less is More: Clustered Cross-Covariance Control for Offline RL
Source: arXiv:2601.20765 source file (2026-01-31)
Supplement: Supplementary file 1 [file LayerNorm.tex]

% \section{Normalization’s Effect on NTK}
\section{The Impact of Normalization on Neural Tangent Kernel}\label{app:ln}

This analysis demonstrates that removing  Normalization modules can lead to Q-value divergence and feature rank collapse, as rigorously established through Neural Tangent Kernel (NTK) theory. Building on the theoretical framework of \citep{yue2023understanding}, we provide convergence guarantees for normalization-equipped networks.

Considering a simple situation, two-layer MLP where input $\mathbf{x} = (\mathbf{s}, \mathbf{a}) \in \mathbb{R}^{d_\text{in}}$ flows through a hidden layer of width $d$. The model parameters consist of $\mathbf{U} = [\mathbf{u}_1, \dots, \mathbf{u}_d]^\top \in \mathbb{R}^{d \times d_\text{in}}$, $\mathbf{c} \in \mathbb{R}^d$, and $\mathbf{v} \in \mathbb{R}^d$. The output function (excluding bias due to constant gradient effects) is:
$$ g_{\boldsymbol{\theta}}(\mathbf{x}) = \sum_{k=1}^d v_k \cdot \mathrm{Var}rho(\mathbf{u}_k^\top \mathbf{x} + c_k), $$
where $\mathrm{Var}rho(\cdot)$ denotes the ReLU activation.

\begin{lemma}[NTK Divergence without Normalization]\label{lemma:w/o-ln}
    For any input $\mathbf{x}$ and parameters $\boldsymbol{\theta}$ where $\nabla_{\boldsymbol{\theta}} g_{\boldsymbol{\theta}}(\mathbf{x}) \neq \mathbf{0}$, the NTK satisfies:
$$
\lim_{\eta \to \infty} k_{\text{NTK}}(\mathbf{x}, \eta \mathbf{x}) = \Omega(\eta) \to \infty.
$$
\end{lemma}
% **Theorem 1 (NTK Divergence without Normalization).** *

\begin{proof}
Let $h_k = \mathbf{u}_k^\top \mathbf{x} + c_k$. By assumption, at least one neuron has $h_k > 0$; denote this active set by $\mathcal{A}$. For $\eta \gg 1$ (selecting sign such that $\mathbf{u}_k^\top \mathbf{x} > 0$), gradients for $k \in \mathcal{A}$ are:
$$
\begin{aligned}
\frac{\partial g}{\partial v_k}\Big|_{\mathbf{x}} &= h_k, \\
\frac{\partial g}{\partial \mathbf{u}_k}\Big|_{\mathbf{x}} &= v_k \mathbf{x}, \\
\frac{\partial g}{\partial c_k}\Big|_{\mathbf{x}} &= v_k,
\end{aligned}
\quad
\begin{aligned}
\frac{\partial g}{\partial v_k}\Big|_{\eta\mathbf{x}} &= \eta \mathbf{u}_k^\top \mathbf{x} + c_k, \\
\frac{\partial g}{\partial \mathbf{u}_k}\Big|_{\eta\mathbf{x}} &= \eta v_k \mathbf{x}, \\
\frac{\partial g}{\partial c_k}\Big|_{\eta\mathbf{x}} &= v_k.
\end{aligned}
$$
The inner product for active neurons scales as:
$$
\sum_{k \in \mathcal{A}} \left\langle \frac{\partial g(\mathbf{x})}{\partial \boldsymbol{\theta}_k}, \frac{\partial g(\eta\mathbf{x})}{\partial \boldsymbol{\theta}_k} \right\rangle = \eta \left[ (\mathbf{u}_k^\top \mathbf{x})^2 + c_k \mathbf{u}_k^\top \mathbf{x} + v_k^2 \|\mathbf{x}\|^2 \right] + \mathcal{O}(1) = \Theta(\eta).
$$
For inactive neurons ($\mathcal{I} = [d] \setminus \mathcal{A}$), gradients vanish as $\eta \to \infty$:
$$
\forall k \in \mathcal{I}, \quad \lim_{\eta \to \infty} \left\langle \frac{\partial g(\mathbf{x})}{\partial \boldsymbol{\theta}_k}, \frac{\partial g(\eta\mathbf{x})}{\partial \boldsymbol{\theta}_k} \right\rangle = 0.
$$
Thus, the NTK grows linearly with scaling:
$$
k_{\text{NTK}}(\mathbf{x}, \eta \mathbf{x}) = \sum_{k=1}^d \left\langle \nabla_{\boldsymbol{\theta}_k} g(\mathbf{x}), \nabla_{\boldsymbol{\theta}_k} g(\eta\mathbf{x}) \right\rangle = \Theta(\eta) \to \infty \quad \square.
$$
\end{proof}

For Normalization-augmented networks, the forward pass becomes:
$$
g_{\boldsymbol{\theta}}(\mathbf{x}) = \mathbf{v}^\top \mathrm{Var}rho\left( \ell(\mathbf{Ux} + \mathbf{c}) \right),
$$
where $\ell(\cdot)$ is  Normalization:
$$
\ell(\mathbf{z}) = \sqrt{d} \cdot \frac{\mathbf{z} - d^{-1}(\mathbf{1}^\top \mathbf{z})\mathbf{1}}{\|\mathbf{z} - d^{-1}(\mathbf{1}^\top \mathbf{z})\mathbf{1}\|_2},
$$
Note $\ell(\eta \mathbf{z}) = \ell(\mathbf{z})$ due to scale invariance. The gradient operator $\ell'(\mathbf{z})$ is:
$$
\ell'(\mathbf{z}) = \sqrt{d} \left( \frac{\mathbf{P}}{\|\mathbf{Pz}\|_2} - \frac{\mathbf{Pz} \mathbf{z}^\top \mathbf{P}}{\|\mathbf{Pz}\|_2^3} \right), \quad \mathbf{P} = \mathbf{I} - d^{-1}\mathbf{11}^\top,
$$

\begin{lemma}[Normalization-Controlled NTK]\label{lemma:w/-ln}
For any $\mathbf{x}, \mu \in \mathbb{R}^{d_\text{in}}$ and parameters $\boldsymbol{\theta}$, there exists $C(\boldsymbol{\theta}, \mathbf{x}, \mu) < \infty$ such that
$$
\sup_{\eta \geq 0} \, k_{\text{NTK}}(\mathbf{x}, \mathbf{x} + \eta \mu) \leq C.
$$    
\end{lemma}

\begin{proof}
Let \(\mathbf{y}_\eta = \mathbf{x} + \eta \mu\). The parameter gradients are:

\[\begin{aligned}
\nabla_{\mathbf{v}} g_{\boldsymbol{\theta}}(\mathbf{y}_\eta) &= \mathrm{Var}rho(\ell(\mathbf{Uy}_\eta + \mathbf{c})) \\
\nabla_{\mathbf{c}} g_{\boldsymbol{\theta}}(\mathbf{y}_\eta) &= \left[ \mathbf{v}^\top \odot \mathrm{Var}rho'(\ell(\mathbf{Uy}_\eta + \mathbf{c})) \right] \ell'(\mathbf{Uy}_\eta + \mathbf{c}) \\
\nabla_{\mathbf{U}} g_{\boldsymbol{\theta}}(\mathbf{y}_\eta) &= \nabla_{\mathbf{c}} g_{\boldsymbol{\theta}}(\mathbf{y}_\eta) \cdot \mathbf{y}_\eta^\top 
\end{aligned}\]

As \(\eta \to \infty\),  Normalization's scale invariance implies:
\[\mathbf{Uy}_\eta + \mathbf{c} = \eta\mathbf{U}\mu + \mathcal{O}(1) \implies \ell(\mathbf{Uy}_\eta + \mathbf{c}) \to \ell(\mathbf{U}\mu)\]
since \(\ell(\lambda\mathbf{z}) = \ell(\mathbf{z})\) for any \(\lambda > 0\). Gradient limits become:

\[\begin{aligned}
\lim_{\eta \to \infty} \nabla_{\mathbf{v}} g_{\boldsymbol{\theta}}(\mathbf{y}_\eta) &= \mathrm{Var}rho(\ell(\mathbf{U}\mu)) \\
\lim_{\eta \to \infty} \nabla_{\mathbf{c}} g_{\boldsymbol{\theta}}(\mathbf{y}_\eta) &= \mathbf{0} \\
\lim_{\eta \to \infty} \nabla_{\mathbf{U}} g_{\boldsymbol{\theta}}(\mathbf{y}_\eta) &= \left[ \mathbf{v}^\top \odot \mathrm{Var}rho'(\ell(\mathbf{U}\mu)) \right] \ell'(\mathbf{U}\mu) \cdot \mathbf{y}_\eta^\top 
= \mathcal{O}(1) \cdot \mathbf{y}_\eta^\top 
\end{aligned}\]

For the Jacobian term:
\[\ell'(\mathbf{z}) = \sqrt{d} \left( \frac{\mathbf{P}}{\|\mathbf{Pz}\|_2} - \frac{\mathbf{Pz} \mathbf{z}^\top \mathbf{P}}{\|\mathbf{Pz}\|_2^3} \right), \quad \mathbf{P} = \mathbf{I} - d^{-1}\mathbf{11}^\top\]
When \(\mathbf{z} = \mathbf{U}\mathbf{y}_\eta + \mathbf{c}\):
\[\begin{aligned}
\ell'(\mathbf{z}) &\sim \eta^{-1} \ell'(\mathbf{U}\mu) \\
\nabla_{\mathbf{U}} g_{\boldsymbol{\theta}}(\mathbf{y}_\eta) &\sim \eta^{-1} \left[ \mathbf{v}^\top \odot \mathrm{Var}rho'(\ell(\mathbf{U}\mu)) \right] \ell'(\mathbf{U}\mu) \cdot (\eta \mu)^\top \\
&= \left[ \mathbf{v}^\top \odot \mathrm{Var}rho'(\ell(\mathbf{U}\mu)) \right] \ell'(\mathbf{U}\mu) \cdot \mu^\top
\end{aligned}\]
All gradients converge to finite values. The NTK inner product \(\langle \nabla_{\boldsymbol{\theta}} g(\mathbf{x}), \nabla_{\boldsymbol{\theta}} g(\mathbf{y}_\eta) \rangle\) remains bounded for \(\eta \in [0, \infty)\), with \(C\) depending only on \(\boldsymbol{\theta}\), \(\mathbf{x}\), and \(\mu\). 
\end{proof}

Lemma \ref{lemma:w/o-ln} establishes that Q-value extrapolation without Normalization causes unbounded NTK growth, while Lemma \ref{lemma:w/-ln} confirms Normalization maintains NTK stability during input scaling.

\section{NTK infinite}

\begin{theorem}[Linear Growth of the NTK Along a Direction]
Consider a two-layer ReLU network
\[
g_\theta(x) = \sum_{i=1}^d v_i \,\sigma(u_i^\top x + c_i), 
\qquad \sigma(t) = \max\{0, t\},
\]
with parameters $u_i \in \mathbb{R}^n$, $v_i, c_i \in \mathbb{R}$. 
The Neural Tangent Kernel (NTK) is defined as
\[
K_\theta(x, x') = \sum_{i=1}^d \left\langle \nabla_{\!(v_i, u_i, c_i)} g_\theta(x), \; \nabla_{\!(v_i, u_i, c_i)} g_\theta(x') \right\rangle.
\]
Let $w \in \mathbb{R}^n$ be a unit vector and define $x_k := x + k w$. 
If there exists at least one neuron index $j$ such that
\[
u_j^\top x + c_j > 0
\quad\text{and}\quad
u_j^\top w > 0,
\]
then there exist constants $c > 0$ and $C < \infty$, independent of $k$, such that
\[
K_\theta(x, x_k) \ge c\,k - C.
\]
In particular,
\[
\lim_{k \to \infty} K_\theta(x, x + k w) = \Omega(k) \to \infty.
\]
\end{theorem}

\begin{proof}
For neuron $i$, define the pre-activation
\[
h_i(z) := u_i^\top z + c_i.
\]
The gradients of $g_\theta$ at $z$ with respect to its parameters are
\[
\frac{\partial g}{\partial v_i}(z) = \sigma(h_i(z)), \quad
\frac{\partial g}{\partial u_i}(z) = v_i\,\mathbf{1} \{h_i(z) > 0\}\, z, \quad
\frac{\partial g}{\partial c_i}(z) = v_i\,\mathbf{1} \{h_i(z) > 0\}.
\]

Let $j$ be a neuron satisfying the assumptions. Then:
% \begin{itemize}
We obtain
$h_j(x) > 0$ implies neuron $j$ is active at $x$, and
$u_j^\top w > 0$ ensures $h_j(x_k) = h_j(x) + k(u_j^\top w) > 0$ for all sufficiently large $k$.
% \end{itemize}
Thus for large $k$,
\[
\sigma(h_j(x_k)) = h_j(x) + k(u_j^\top w) = k(u_j^\top w) + O(1).
\]

The contribution of neuron $j$ to the NTK is
\[
\begin{aligned}
I_j(k)
&= \left\langle \nabla g_j(x), \nabla g_j(x_k) \right\rangle \\
&= \underbrace{\sigma(h_j(x))\,\sigma(h_j(x_k))}_{(A)}
+ \underbrace{v_j^2\,\mathbf{1}\{h_j(x) > 0\}\,\mathbf{1}\{h_j(x_k) > 0\} \, x^\top(x_k)}_{(B)}
+ \underbrace{v_j^2\,\mathbf{1}\{h_j(x) > 0\}\,\mathbf{1}\{h_j(x_k) > 0\}}_{(C)}.
\end{aligned}
\]
where
(A) grows linearly: 
    \[
    (A) = \sigma(h_j(x))\,[k(u_j^\top w) + O(1)] = (\sigma(h_j(x))\,u_j^\top w)\,k + O(1),
    \]
    where the coefficient is strictly positive by assumption.
(B) is $O(k)$ and nonnegative.
(C) is $O(1)$ and nonnegative.
% \end{itemize}
Hence there exist constants $c>0$ and $C<\infty$ such that
\[
I_j(k) \ge c\,k - C.
\]
Since $K_\theta(x, x_k)$ is the sum of nonnegative neuron contributions,
\[
K_\theta(x, x_k) \ge I_j(k) \ge c\,k - C,
\]
which proves the claim.
\end{proof}

\begin{remark}
The condition $u_j^\top x + c_j > 0$ and $u_j^\top w > 0$ is necessary for linear growth. 
If all active neurons at $x$ satisfy $u_i^\top w \le 0$, or if no neuron is active at $x$, then $K_\theta(x, x_k)$ can remain bounded or vanish. 
Under continuous random initialization of $(u_i, c_i)$, for any fixed $x$ and $w$ the condition holds almost surely, so $\Omega(k)$ growth occurs with probability $1$.
\end{remark}

\begin{lemma}[NTK Growth for $L$-Layer ReLU Networks]
Consider an $L$-hidden-layer ReLU network:
\[
a^{(0)}(x) = x,\quad
z^{(\ell)}(x) = W_\ell a^{(\ell-1)}(x) + b_\ell,\quad
a^{(\ell)}(x) = \sigma\!\big(z^{(\ell)}(x)\big),\quad
g_\theta(x) = v^\top a^{(L)}(x) + b_{L+1},
\]
with $\sigma(t) = \max\{0,t\}$. Let $w \in \mathbb{R}^n$ be a unit vector and $x_k := x + k w$. 
If there exist indices $(j_1,\dots,j_L)$ such that:
\begin{enumerate}
\item $z^{(1)}_{j_1}(x) > 0$ and $(W_1)_{j_1,:} w > 0$,
\item $z^{(\ell)}_{j_\ell}(x) > 0$ and $(W_\ell)_{j_\ell,j_{\ell-1}} > 0$ for $\ell = 2,\dots,L$,
\end{enumerate}
then there exist constants $c>0$ and $C<\infty$ (independent of $k$) such that
\[
K_\theta(x, x_k) \ge c\,k^{L} - C.
\]
In particular, $\lim_{k\to\infty} K_\theta(x, x + k w) = \Omega(k^{L}) \to \infty$.
\end{lemma}

\begin{proof}
Along the path $(j_1,\dots,j_L)$, condition (1) implies
\[
a^{(1)}_{j_1}(x_k) = \sigma\!\big(z^{(1)}_{j_1}(x) + k\,(W_1)_{j_1,:} w\big) 
= \Theta(k) \quad (k\to\infty).
\]
By induction, using condition (2) and ReLU's positive homogeneity,
\[
a^{(\ell)}_{j_\ell}(x_k) = \Theta(k^{\ell}) \quad \text{for all } \ell=1,\dots,L.
\]
In particular, $a^{(L)}_{j_L}(x_k) = \Theta(k^L)$ and $a^{(L)}_{j_L}(x) > 0$.

The gradient w.r.t.\ $v_{j_L}$ satisfies 
$\frac{\partial g_\theta(z)}{\partial v_{j_L}} = a^{(L)}_{j_L}(z)$, hence its NTK contribution is
\[
a^{(L)}_{j_L}(x) \cdot a^{(L)}_{j_L}(x_k) = c\,k^{L} + O(1)
\]
with $c = a^{(L)}_{j_L}(x) > 0$. Since the NTK sums nonnegative contributions over parameters,
$K_\theta(x,x_k) \ge c\,k^{L} - C$, proving the claim.
\end{proof}
