# Supplementary material for: Less is More: Clustered Cross-Covariance Control for Offline RL
Source: arXiv:2601.20765 source file (2026-01-31)
Supplement: Supplementary file 2 [file TDLoss-v1-s2.tex]

\section{TDLoss-v1-s2}

\begin{lemma}[Variance of TD Error Along a Direction]
Let $Q_\theta(x)$ be the predicted Q-value parameterized by $\theta$, and denote $x_k := x + k w$ where $w$ is a unit vector. Suppose that for in-distribution state-action pairs $(s,a)$, the Bellman error is minimized so that $Q_\theta(s,a) \approx Q_\theta^\ast(s,a)$. For an out-of-distribution (OOD) perturbation along $w$, a first-order Taylor expansion yields
\[
Q_\theta(x_k) \approx Q_\theta(x) + k \langle w, \nabla_x Q_\theta(x) \rangle.
\]
Let $\Sigma_t := \mathrm{Var}(\nabla_x Q_{\theta_t}(x))$ and $\Sigma_{t+1} := \mathrm{Var}(\nabla_x Q_{\theta_{t+1}}(x'))$ be the sample gradient covariance matrices, and let 
\[
C := \mathrm{Cov}\big(\nabla_x Q_{\theta_t}(x'), \nabla_x Q_{\theta_{t+1}}(x)\big).
\]
For $x=(s,a)\sim D$ and $x'=(s',a')\sim D$, we have
\[
\mathrm{Var}[\delta_{t+1}] 
= k_2^2 \gamma^2\, w_2^\top \Sigma_t \, w_2 
+ k_1^2\, w_1^\top \Sigma_{t+1} \, w_1
- 2\gamma k_1 k_2\, w_2^\top C\, w_1,
\]
where $k_1, k_2$ are the perturbation magnitudes along $w_1, w_2$, respectively.
\end{lemma}

\begin{proof}
Starting from
\[
\delta_{t+1} = R + \gamma Q_{\theta_t}(x' + k_2 w_2) - Q_{\theta_{t+1}}(x + k_1 w_1),
\]
and applying the first-order Taylor approximation
\[
Q_\theta(z + k w) \approx Q_\theta(z) + k \langle w, \nabla_z Q_\theta(z) \rangle,
\]
the variance becomes
\[
\mathrm{Var}[\delta_{t+1}] 
\approx \mathrm{Var}\!\left( \gamma k_2 \langle w_2, \nabla_x Q_{\theta_t}(x') \rangle 
 - k_1 \langle w_1, \nabla_x Q_{\theta_{t+1}}(x) \rangle \right).
\]
Expanding the variance of a difference yields
\[
\gamma^2 k_2^2\, \mathrm{Var}(\langle w_2, \nabla_x Q_{\theta_t}(x') \rangle) 
+ k_1^2\, \mathrm{Var}(\langle w_1, \nabla_x Q_{\theta_{t+1}}(x) \rangle) 
- 2\gamma k_1 k_2\, \mathrm{Cov}(\langle w_2, \nabla_x Q_{\theta_t}(x') \rangle, \langle w_1, \nabla_x Q_{\theta_{t+1}}(x) \rangle),
\]
which can be written compactly using $\Sigma_t$, $\Sigma_{t+1}$ and $C$ as in the lemma statement.
\end{proof}

\begin{corollary}[Special Case: Isotropic Gradients and Same Direction Perturbation]
If $w_1=w_2=w$, $\|w\|_2=1$, and the gradient covariances are isotropic, i.e.
\[
\Sigma_t \approx \frac{1}{d} \,\mathrm{Gram}(X', X')\, I, 
\quad
\Sigma_{t+1} \approx \frac{1}{d} \,\mathrm{Gram}(X, X)\, I,
\quad
C \approx \frac{1}{d} \,\mathrm{Gram}(X', X)\, I,
\]
then
\[
\mathrm{Var}[\delta_{t+1}]
\approx \frac{\gamma^2 k_2^2}{d} \,\mathrm{tr}[\mathrm{Gram}(X',X')] 
+ \frac{k_1^2}{d} \,\mathrm{tr}[\mathrm{Gram}(X,X)]
- \frac{2\gamma k_1 k_2}{d} \,\mathrm{tr}[\mathrm{Gram}(X',X)].
\]
In particular, the $-2\gamma\,\mathrm{tr}[\mathrm{Gram}(X',X)]$ term emerges from the cross-covariance $-2\gamma k_1 k_2\, w^\top C w$ under isotropy.
\end{corollary}

\begin{theorem}[Subspace Manifold Separation reduces the TD cross term]
Let $\psi(x)$ be whitened gradient features. Suppose samples in cluster $c$ and $d$
concentrate around linear subspaces $U_c,U_d$ with approximately isotropic covariances
$\sigma_c^2P_{U_c},\sigma_d^2P_{U_d}$. For a minibatch drawing $X$ from $c$ and $X'$ from $d$,
\[
\mathbb{E}\,\mathcal{R}(X',X)\ \propto\ \operatorname{tr}(P_{U_c}P_{U_d})
\ =\ \sum_{i=1}^{k_\star}\cos^2\theta_i(U_c,U_d),
\]
where $\{\theta_i\}$ are principal angles and $k_\star=\min(\dim U_c,\dim U_d)$.
Hence choosing cluster pairs with larger principal angles minimizes the TD cross term.
\end{theorem}

\begin{theorem}[CCA bound for general distributions]
Let $\Sigma_{12}=\operatorname{Cov}(\psi(X'),\psi(X))$ and 
$\{\rho_i\}_{i=1}^r$ be canonical correlations. Then for a minibatch of sizes $m,m'$,
\[
\big|\mathbb{E}\,\mathcal{R}(X',X)\big|
\ \le\ \frac{1}{\sqrt{mm'}}\|\Sigma_{12}\|_\ast
\ =\ \frac{1}{\sqrt{mm'}}\sum_{i=1}^r \rho_i
\ \le\ \sqrt{\frac{r}{mm'}}.
\]
Dataset splitting that reduces $r$ and $\{\rho_i\}$ (by pairing decorrelated clusters) 
tightens the bound and suppresses the harmful TD cross term.
\end{theorem}

\begin{algorithm}[H]
\caption{Manifold Separation for TD Batching}
\begin{algorithmic}[1]
\State Collect features $\phi_\theta(x)$, estimate $\mu,\Sigma$, whiten to get $\psi(x)$.
\State Cluster $\{\psi(x)\}$ into $K$ groups; per cluster, fit PCA to get subspace $U_c$.
\State For each pair $(c,d)$, compute $A_{cd}=\|P_{U_c}P_{U_d}\|_F^2$.
\State For each minibatch: pick cluster $c$ for $X$, sample $X'$ from cluster $d$ with prob. $\pi(d|c)\propto e^{-\beta A_{cd}}$.
\State (Optional) Enforce $\mathcal{R}(X',X)\le \epsilon$ by swapping samples; or add $\lambda\,\mathcal{R}(X',X)$ to the loss.
\State Every $T$ steps, update $\psi,U_c,A_{cd}$ with the latest $\theta$.
\end{algorithmic}
\end{algorithm}
