# Supplementary material for: Less is More: Clustered Cross-Covariance Control for Offline RL
Source: arXiv:2601.20765 source file (2026-01-31)
Supplement: Supplementary file 3 [file TDLoss-v2-s1.tex]

% =========================
% TD Loss (offline RL, full-input x, centered moments, no \paragraph)
% =========================

\section{TD Loss v2 (Offline RL; full-input $x$)}

We keep all quantities at iteration $k$ and use a fixed offline dataset $D$ of transitions
$\zeta=(s,a,r,s')\sim D$. Let $x=(s,a)$ and $x'=(s',a')$.

In tabular Q-learning, the TD error and update are
\begin{align}
\delta &= r + \gamma \max_{a'} Q(s',a') - Q(s,a),
\label{eq:td_error_tabular_x}
\\
Q(s,a) &\leftarrow Q(s,a) + \alpha\,\delta,
\label{eq:q_update_x}
\end{align}
where $\alpha$ is the learning rate.

For offline RL with a lagged/target network, let current parameters be $\theta_k$ and lagged parameters be $\theta_{k-1}$ (or a Polyak average). The TD error and squared loss at iteration $k$ are
\begin{align}
\delta_k &= r + \gamma \max_{a'} Q(s',a';\,\theta_{k-1}) - Q(s,a;\,\theta_k)
= r + \gamma \max_{a'} Q(x';\,\theta_{k-1}) - Q(x;\,\theta_k),
\label{eq:td_error_offline_x}
\\
\mcal{L}(\theta_k) &= \E\!\big[\tfrac{1}{2}\,\delta_k^2\big],
\label{eq:loss_offline_x}
\end{align}
and the variance decomposition identity is used only as an identity:
\begin{align}
\E[\delta_k^2] = \big(\E[\delta_k]\big)^2 + \mathrm{Var}(\delta_k).
\label{eq:var_decomp_x}
\end{align}
Expectations/variances are w.r.t.\ $\zeta\sim D$ (and any auxiliary randomness made explicit below).

Define the full-input gradient and dimension
\begin{align}
\phi_{\theta}(x) &\coloneqq \nabla_{x}\,Q_{\theta}(x),
\label{eq:phi_def_x}
\\
d &\coloneqq \mathrm{dim}(x).
\label{eq:dim_def_x}
\end{align}
For a unit direction $w\in\mathbb{R}^d$ with $\|w\|=1$ and a small displacement $\kappa\in\mathbb{R}$, a first-order expansion gives
\begin{align}
Q_{\theta}(x+\kappa w) \;\approx\; Q_{\theta}(x) + \kappa\, w^{\top}\phi_{\theta}(x),
\label{eq:taylor_x}
\end{align}
so that
\begin{align}
\mathrm{Var}\!\big(Q_{\theta}(x+\kappa w)\big)
&\approx \mathrm{Var}\!\big(Q_{\theta}(x)\big)
+ \kappa^{2}\, w^{\top}\,\mathrm{Var}\!\big(\phi_{\theta}(x)\big)\,w
+ 2\kappa\,\mathrm{Cov}\!\big(Q_{\theta}(x),\,w^{\top}\phi_{\theta}(x)\big).
\label{eq:var_q_general_x}
\end{align}
Keeping only the incremental variance and neglecting the covariance term,
\begin{align}
\Delta\mathrm{Var}
:= \mathrm{Var}\!\big(Q_{\theta}(x+\kappa w)\big) - \mathrm{Var}\!\big(Q_{\theta}(x)\big)
\;\approx\; \kappa^{2}\, w^{\top}\,\mathrm{Var}\!\big(\phi_{\theta}(x)\big)\,w.
\label{eq:delta_var_x}
\end{align}
Averaging over $w\sim\mathrm{Unif}(S^{d-1})$ and using $\E_{w}[\langle w,u\rangle^{2}]=\|u\|^{2}/d$ yields
\begin{align}
\E_{w}[\Delta\mathrm{Var}]
\;\approx\; \frac{\kappa^{2}}{d}\,\mathrm{tr}\!\big(\mathrm{Var}(\phi_{\theta}(x))\big).
\label{eq:avg_w_x}
\end{align}

Keep all quantities at iteration $k$ and a single transition $\zeta=(s,a,r,s')$.
Define the full-input gradients of the target (lagged) and current networks:
\begin{align}
g^{\mathrm{tar}}_{k-1}(x') &:= \nabla_{x'} Q_{\theta_{k-1}}(x'),
\qquad
g^{\mathrm{on}}_{k}(x) \;:=\; \nabla_{x}  Q_{\theta_{k}}(x).
\label{eq:g_defs_x}
\end{align}
Consider small shifts $x+\kappa_{1}w_{1}$ and $x'+\kappa_{2}w_{2}$ with $w_{1},w_{2}\sim\mathrm{Unif}(S^{d-1})$.
A first-order approximation of the TD error variance is
\begin{align}
\mathrm{Var}(\delta_{k})
&\approx \mathrm{Var}(r)
+ \gamma^{2}\kappa_{2}^{2}\, w_{2}^{\top}\,\mathrm{Var}\!\big(g^{\mathrm{tar}}_{k-1}(x')\big)\,w_{2}
+ \kappa_{1}^{2}\, w_{1}^{\top}\,\mathrm{Var}\!\big(g^{\mathrm{on}}_{k}(x)\big)\,w_{1}
\notag\\[-0.25em]
&\hspace{2em}
- 2\gamma\,\kappa_{1}\kappa_{2}\, w_{2}^{\top}\,\mathrm{Cov}\!\big(g^{\mathrm{tar}}_{k-1}(x'),\,g^{\mathrm{on}}_{k}(x)\big)\,w_{1}.
\label{eq:var_td_x}
\end{align}
If $w_{2}\perp w_{1}$ and the cross term is weak, the covariance term can be neglected. Averaging over $w_{1},w_{2}$ gives
\begin{align}
\E_{w_{1},w_{2}}\big[\mathrm{Var}(\delta_{k})\big]
\;\approx\;
\mathrm{Var}(r)
+ \frac{\gamma^{2}\kappa_{2}^{2}}{d}\,\mathrm{tr}\!\big(\mathrm{Var}(g^{\mathrm{tar}}_{k-1})\big)
+ \frac{\kappa_{1}^{2}}{d}\,\mathrm{tr}\!\big(\mathrm{Var}(g^{\mathrm{on}}_{k})\big)
- \frac{2\gamma\kappa_{1}\kappa_{2}}{d}\,\mathrm{tr}\!\big(\mathrm{Cov}(g^{\mathrm{tar}}_{k-1},g^{\mathrm{on}}_{k})\big).
\label{eq:avg_var_td_x}
\end{align}

For a mini-batch $X=\{x_i\}_{i=1}^n$ and $X'=\{x'_i\}_{i=1}^n$, define gradient matrices
\begin{align}
\Phi^{\mathrm{on}}_{k}(X) &:= \big[g^{\mathrm{on}}_{k}(x_1),\dots,g^{\mathrm{on}}_{k}(x_n)\big]\in\mathbb{R}^{d\times n},
\qquad
\Phi^{\mathrm{tar}}_{k-1}(X') := \big[g^{\mathrm{tar}}_{k-1}(x'_1),\dots,g^{\mathrm{tar}}_{k-1}(x'_n)\big].
\label{eq:Phi_defs_x}
\end{align}
Let the column means be
$\mu^{\mathrm{on}}=\tfrac{1}{n}\sum_{i} g^{\mathrm{on}}_{k}(x_i)$ and
$\mu^{\mathrm{tar}}=\tfrac{1}{n}\sum_{i} g^{\mathrm{tar}}_{k-1}(x'_i)$,
and the centered matrices
$\tilde\Phi^{\mathrm{on}}_{k}=\Phi^{\mathrm{on}}_{k}-\mu^{\mathrm{on}}\mathbf{1}^{\top}$,
$\tilde\Phi^{\mathrm{tar}}_{k-1}=\Phi^{\mathrm{tar}}_{k-1}-\mu^{\mathrm{tar}}\mathbf{1}^{\top}$.
The empirical centered traces satisfy
\begin{align}
\mathrm{tr}\!\big(\mathrm{Var}(g^{\mathrm{on}}_{k})\big)
&\approx \tfrac{1}{n}\,\|\tilde\Phi^{\mathrm{on}}_{k}\|_{F}^{2}
= \tfrac{1}{n}\,\mathrm{tr}\!\big(\tilde\Phi^{\mathrm{on}}_{k}\tilde\Phi^{\mathrm{on}\,\top}_{k}\big),
\label{eq:trace_var_on_x}
\\
\mathrm{tr}\!\big(\mathrm{Var}(g^{\mathrm{tar}}_{k-1})\big)
&\approx \tfrac{1}{n}\,\|\tilde\Phi^{\mathrm{tar}}_{k-1}\|_{F}^{2}
= \tfrac{1}{n}\,\mathrm{tr}\!\big(\tilde\Phi^{\mathrm{tar}}_{k-1}\tilde\Phi^{\mathrm{tar}\,\top}_{k-1}\big),
\label{eq:trace_var_tar_x}
\\
\mathrm{tr}\!\big(\mathrm{Cov}(g^{\mathrm{tar}}_{k-1},\,g^{\mathrm{on}}_{k})\big)
&\approx \tfrac{1}{n}\,\mathrm{tr}\!\big(\tilde\Phi^{\mathrm{tar}\,\top}_{k-1}\,\tilde\Phi^{\mathrm{on}}_{k}\big).
\label{eq:trace_cov_on_tar_x}
\end{align}
Substituting \eqref{eq:trace_var_on_x}--\eqref{eq:trace_cov_on_tar_x} into \eqref{eq:avg_var_td_x} gives a data-dependent approximation to the expected TD error variance at iteration $k$.

% Note: For Double DQN, replace the $\max$-branch accordingly and assume the selected action branch is locally stable so that the subgradient w.r.t.\ $x'$ is well defined in a small neighborhood.
