# Supplementary material for: Less is More: Clustered Cross-Covariance Control for Offline RL
Source: arXiv:2601.20765 source file (2026-01-31)
Supplement: Supplementary file 4 [file app_Cluster.tex]

\section{Method: Two-Sided Cluster-Pair Stratified Sampling (Parallel Mini-batch)}
\label{sec:method-cluster-stratified}

% \paragraph{Setup.}
Offline dataset $\mathcal{D}=\{(s_i,a_i,r_i,s'_i)\}_{i=1}^N$. Let $x_i=(s_i,a_i)$ and $x'_i=(s'_i,a'_i)$ (e.g., $a'_i=\arg\max_a Q_{\bar\theta}(s'_i,a)$ or sampled from the current policy). Define a representation $\phi_\theta(x)\in\mathbb{R}^m$ (e.g., the penultimate-layer activation; standardize/whiten in practice).

% \paragraph{Two-sided clustering.}
Run k-means (or spherical k-means) separately on $\{\phi_\theta(x_i)\}$ and $\{\phi_\theta(x'_i)\}$ to obtain clusters
$\{S_c\}_{c=1}^{K}$ and $\{S'_{c'}\}_{c'=1}^{K'}$.
Each transition $i$ is assigned to a \emph{cluster pair} $(c'(i),c(i))$ where
\[
\mathcal{I}_{c',c}=\{\,i:\ x'_i\in S'_{c'},\ x_i\in S_c\,\}.
\]

% \paragraph{Cross-time gradient cross-covariance.}
Estimate the next-vs-current gradient cross-covariance on each cluster pair:
\[
g_i=\nabla_x Q_{\theta_t}(x'_i),\quad
h_i=\nabla_x Q_{\theta_{t+1}}(x_i),\quad
\widehat C_{c',c}=\frac{1}{|\mathcal{I}_{c',c}|}\sum_{i\in\mathcal{I}_{c',c}}
\big(g_i-\bar g_{c'}\big)\big(h_i-\bar h_{c}\big)^\top,
\]
with $\bar g_{c'}=\frac{1}{|\mathcal{I}_{c'}|}\sum_{i\in\mathcal{I}_{c'}} g_i$ and
$\bar h_c=\frac{1}{|\mathcal{I}_{c}|}\sum_{i\in\mathcal{I}_{c}} h_i$.
Define a scalar \emph{pairwise alignment score} (smaller is better):
\[
m_{c',c}=\|\widehat C_{c',c}\|_F \quad \text{or} \quad m_{c',c}=\sigma_{\max}(\widehat C_{c',c}).
\]

% \paragraph{Sampling distribution over cluster pairs.}
To reduce the overall cross-time term, draw mini-batches from cluster pairs according to
\begin{align}
\label{eq:softmax-p}
p(c',c)\ \propto\ u(c',c)\,\exp\!\Big(-\tfrac{m_{c',c}}{\tau}\Big),
\end{align}
where $u$ is a baseline (e.g., uniform) and $\tau>0$ is a temperature. In practice we use a mixture $\tilde p=\alpha\,p+(1-\alpha)\,u$ to avoid coverage collapse.

% \paragraph{Objective (unchanged TD) and optional regularization.}
Keep the standard TD loss:
\[
\mathcal{L}_{\text{TD}}=\mathbb{E}_{(s,a,r,s')\sim \tilde p}\big[\,(r+\gamma\,\text{target}(s')-Q_\theta(s,a))^2\,\big].
\]
Optionally add an explicit cross-time penalty
$\mathcal{L}_{\text{cov}}=\lambda \sum_{c',c}\omega_{c',c}\,m_{c',c}^2$
or $\lambda \sum_{c',c}\omega_{c',c}\,\sigma_{\max}(\widehat C_{c',c})^2$.

% \paragraph{Why it helps (sketch).}
Let $m_{c',c}\ge |w_2^\top \widehat C_{c',c} w_1|$. Then
\[
\big|w_2^\top \widehat C w_1\big|
=\Big|\sum_{c',c} p(c',c)\,w_2^\top \widehat C_{c',c} w_1\Big|
\le \sum_{c',c} p(c',c)\,m_{c',c}.
\]
Minimizing $\sum_{c',c} p\, m_{c',c} + \tau\,\mathrm{KL}(p\|u)$ over $p\in\Delta$ yields \eqref{eq:softmax-p}, thus tightening an upper bound on the cross-time term. Matrix concentration for sub-Gaussian gradients gives stability of $\widehat C_{c',c}$ estimates with sufficient probe samples.

% \Statex 等

\begin{algorithm}[t]
\caption{Parallel Two-Sided Cluster-Pair Stratified Sampling for Offline Q-learning}
\label{alg:parallel-cluster}
\begin{algorithmic}[1]
\Require Dataset $\mathcal{D}$; total batch size $B_{\mathrm{tot}}$; number of workers $P$; clusters $(K,K')$; refresh period $T$; temperature $\tau$; mix $\alpha$
\State Initialize critic $Q_\theta$; set target parameters $\bar\theta \gets \theta$
\For{$t=1,2,\dots$}
  \If{$t \bmod T = 0$} \Comment{Periodic refresh}
    \State Compute features $\phi_\theta(x_i)$ and $\phi_\theta(x'_i)$; normalize to get $\psi_i,\psi'_i$
    \State Run K-means on $\{\psi_i\}$ into $\{S_c\}_{c=1}^{K}$; on $\{\psi'_i\}$ into $\{S'_{c'}\}_{c'=1}^{K'}$
    \State Build index sets $\mathcal{I}_{c',c} \gets \{\,i : \psi'_i \in S'_{c'},\ \psi_i \in S_c\,\}$ for all $(c',c)$
    \State From a probe pool, estimate affinities $\widehat C_{c',c}$ and scores $m_{c',c}$
    \State Compute sampling probs over all pairs by softmax:
           \[
             p(c',c) \gets \frac{\exp\!\big(-m_{c',c}/\tau\big)}{\sum_{\bar c',\bar c}\exp\!\big(-m_{\bar c',\bar c}/\tau\big)},\quad
             \tilde p(c',c) \gets \alpha\, p(c',c) + (1-\alpha)\, u(c',c)
           \]
           where $u(\cdot)$ is the uniform distribution on pairs.
  \EndIf
  \Statex \textbf{(In parallel on $P$ workers)}
  \For{$p \gets 1 \ \mathbf{to}\ P$}
    \State $\mathcal{B}^{(p)} \gets \emptyset$
    \For{$b \gets 1 \ \mathbf{to}\ B_{\mathrm{tot}}/P$}
      \State Sample a pair $(c',c) \sim \tilde p$
      \State Sample index $i$ uniformly from $\mathcal{I}_{c',c}$ (keep $(x_i,x'_i)$ paired)
      \State $\delta_i \gets r_i + \gamma\,\mathrm{target}(s'_i) - Q_\theta(s_i,a_i)$
      \State $\mathcal{B}^{(p)} \gets \mathcal{B}^{(p)} \cup \{i\}$
    \EndFor
    \State $\mathcal{L}^{(p)}_{\mathrm{TD}} \gets \frac{P}{B_{\mathrm{tot}}} \sum_{i \in \mathcal{B}^{(p)}} \delta_i^2$ \Comment{optionally add $+\ \mathcal{L}_{\mathrm{cov}}$}
  \EndFor
  \State All-reduce $\nabla_\theta \sum_{p=1}^P \mathcal{L}^{(p)}_{\mathrm{TD}}$ and update $\theta$
  \State Periodically update target by EMA: $\bar\theta \gets \tau_{\mathrm{EMA}}\theta + (1-\tau_{\mathrm{EMA}})\bar\theta$
\EndFor
\end{algorithmic}
\end{algorithm}

% \paragraph{Practical notes.}
% Typical settings: $B_{\text{tot}}\in[256,1024]$, $P$ by device count; $K,K'\in[50,200]$; refresh $T\in[500,2000]$ steps; temperature $\tau$ annealed from small to large; mix $\alpha\in[0.3,0.7]$. The TD objective remains unchanged; only the sampling distribution is adapted. Each worker samples independently from the same $\tilde p$ and gradients are aggregated via All-Reduce.
