# Supplementary material for: Less is More: Clustered Cross-Covariance Control for Offline RL
Source: arXiv:2601.20765 source file (2026-01-31)
Supplement: Supplementary file 5 [file app_Cross-Transition.tex]

\section{Cross-Transition Coupling and Target Leakage}

\begin{lemma}[Single-step mis-credit assignment under kernel ridge regression]
Let the training set consist of two points $u$ and $v$ with kernel Gram matrix
\begin{equation}
K_{2}=
\begin{pmatrix}
a & b \\
b & c
\end{pmatrix},
\quad a=K(u,u),\; c=K(v,v),\; b=K(u,v),
\end{equation}
and corresponding scalar targets $y=(y_u,y_v)^\top$.  
For $\lambda>0$ define $\alpha=(K_2+\lambda I)^{-1}y$. The kernel ridge predictor at $v$ is
\begin{equation}
\hat f(v) 
= b\alpha_1 + c\alpha_2
= \frac{c(a+\lambda)-b^2}{\Delta}\,y_v
  + \frac{b\lambda}{\Delta}\,y_u,
\label{eq:kridge-v}
\end{equation}
where
\begin{equation}
\Delta = (a+\lambda)(c+\lambda) - b^2.
\end{equation}
Consequently, the contribution of $y_u$ to $\hat f(v)$ equals
\begin{equation}
\theta_{u\to v} = \frac{b\lambda}{\Delta}.
\end{equation}
If $a,c,b$ are $\Theta(1)$ (bounded away from $0$ and $\infty$) and $\lambda=\Theta(1)$, then $\theta_{u\to v}=\Theta(1)$.
\end{lemma}

\begin{proof}
The inverse of $K_2+\lambda I$ is
\begin{equation}
(K_2+\lambda I)^{-1} 
= \frac{1}{\Delta}
\begin{pmatrix}
c+\lambda & -b \\
-b & a+\lambda
\end{pmatrix}.
\end{equation}
Thus 
\[
\alpha_1 = \frac{(c+\lambda)y_u - b y_v}{\Delta},\quad 
\alpha_2 = \frac{-b y_u + (a+\lambda) y_v}{\Delta}.
\]
Substituting into $\hat f(v) = [\,b\ \ c\,]\alpha$ yields \eqref{eq:kridge-v}.
Since $K_2$ is positive semidefinite, $b^2\le ac$ and $\Delta>0$ for $\lambda>0$. If $a,b,c,\lambda=\Theta(1)$ then $\Delta=\Theta(1)$ and $\theta_{u\to v}=\Theta(1)$, proving the claim.
\end{proof}

\begin{lemma}[Bootstrapping amplification and target leakage]
Consider two transitions $(x_1,x_1')$ and $(x_2,x_2')$. Suppose $\hat f$ is obtained via kernel ridge regression and TD targets are
\begin{equation}
y_i = r_i + \gamma\,\hat f(x_i'), \quad 0\le \gamma < 1.
\end{equation}
Let the dependence of $\hat f$ on $(y_1,y_2)$ at $(x_1',x_2')$ be
\begin{equation}
\begin{pmatrix}
\hat f(x_1') \\[2pt] \hat f(x_2')
\end{pmatrix}
= M
\begin{pmatrix}
y_1 \\[2pt] y_2
\end{pmatrix},
\quad M\ge 0.
\end{equation}
Writing $\mathbf f=[\hat f(x_1'),\hat f(x_2')]^\top$ and $\mathbf r=[r_1,r_2]^\top$, the TD equations read
\begin{equation}
\mathbf f = M(\mathbf r + \gamma \mathbf f),
\label{eq:td-matrix}
\end{equation}
with fixed-point solution (if it exists)
\begin{equation}
\mathbf f = (I - \gamma M)^{-1} M \mathbf r.
\label{eq:fixedpoint}
\end{equation}
If $\rho(\gamma M) < 1$, the operator norm satisfies
\begin{equation}
\|(I - \gamma M)^{-1} M\| \ \ge \ \frac{\|M\|}{1-\rho(\gamma M)}.
\end{equation}
As $\rho(\gamma M) \to 1^{-}$, the sensitivity of $\mathbf f$ to $\mathbf r$ diverges. If $\rho(\gamma M)\ge 1$, no stable fixed point is guaranteed.
\end{lemma}

\begin{proof}
From \eqref{eq:td-matrix}, $(I - \gamma M)\mathbf f = M\mathbf r$. If $I-\gamma M$ is invertible, \eqref{eq:fixedpoint} holds. For $\rho(\gamma M) < 1$, the Neumann series gives
\[
(I - \gamma M)^{-1} = \sum_{k=0}^\infty (\gamma M)^k,
\]
hence $\|(I - \gamma M)^{-1}\| \ge \frac{1}{1 - \rho(\gamma M)}$. Multiplying by $\|M\|$ yields the bound. Large constant-order off-diagonal entries of $M$ (cf.\ Lemma~1) ensure $\|M\|=\Theta(1)$, so for typical $\gamma$ the spectral radius $\rho(\gamma M)$ may approach or exceed $1$, causing amplification or instability.
\end{proof}

\paragraph{Discussion.} Lemma~1 shows that large cross-kernel entries $K(x_1',x_2)$ create constant-order cross-label weights $\theta_{u\to v}$. Lemma~2 shows that when such cross-coupling occurs in bootstrapped TD learning, the fixed-point map $(I - \gamma M)^{-1}M$ can amplify these couplings, leading to severe mis-credit assignment and target leakage. In the NTK regime \cite{jacot2018ntk,lee2019wide,xu2020ntk}, the coefficients $M$ are algebraic functions of Gram blocks; your earlier NTK growth result implies these off-diagonal Gram entries can be large when $x_1'$ and $x_2'$ lie in the same ReLU activation cone, hence satisfying the conditions for instability.

\newpage

\newpage
\begin{proposition}[Block-diagonal cross-time covariance under multimodal data]\label{prop:block-diag-crosscov}
Let the offline data distribution be a mixture $D=\sum_{m=1}^M {q}_m D_m$ with ${q}_m>0$ and $\sum_m {q}_m=1$, where $D_m$ is the $m$-th mode (peak).
Define the gradient field $g_t(x):=\nabla_x Q_{\theta_t}(x)$.
For each mode, let
\[
\Sigma_t^{(m)}:=\mathrm{Var}\!\big(g_t(x)\mid x\!\in\!D_m\big),\qquad
\Sigma_{t+1}^{(m)}:=\mathrm{Var}\!\big(g_{t+1}(x)\mid x\!\in\!D_m\big),
\]
and define the cross-time, cross-mode covariance
\[
C_{mn}:=\mathrm{Cov}\!\big(g_t(x')\mid x'\!\in\!D_m,\; g_{t+1}(x)\mid x\!\in\!D_n\big).
\]
Assume there exists $\varepsilon\in[0,1)$ such that for any $m\neq n$ and any unit vectors $u,v$,
\begin{equation}\label{eq:modal-sep}
\big|u^\top C_{mn}\, v\big|
~\le~
\varepsilon\,\sqrt{\big(u^\top \Sigma_t^{(m)} u\big)\big(v^\top \Sigma_{t+1}^{(n)} v\big)}.
\end{equation}
(This captures \emph{modal separation/low similarity}: cross-mode gradient correlation is bounded by $\varepsilon\ll 1$; it is implied, e.g., by sufficiently small NTK similarity across modes.)

Let the overall cross-time covariance be
\[
C~:=~\mathrm{Cov}\!\big(g_t(x'),\,g_{t+1}(x)\big)
~=~\sum_{m,n=1}^M {q}_m{q}_n\,C_{mn}.
\]
Then for any pair of mode indices $(i,j)$ and unit directions $w_j$ (for $x'\!\in\!D_j$) and $w_i$ (for $x\!\in\!D_i$),
\begin{equation}\label{eq:cross-term-bound}
\big|\,w_j^\top C\, w_i\,\big|
~\le~
\pi_i\pi_j\,\varepsilon\,
\sqrt{\big(w_j^\top \Sigma_t^{(j)} w_j\big)\big(w_i^\top \Sigma_{t+1}^{(i)} w_i\big)}
~+~ \sum_{m=1}^M {q}_m^2\,\big|w_j^\top C_{mm} w_i\big|.
\end{equation}
In particular, when $i\neq j$ (cross-mode pairing) and $w_j,w_i$ are chosen within their respective modes,
\[
{\quad
\big|\,w_j^\top C\, w_i\,\big|
~\le~
\pi_i\pi_j\,\varepsilon\,
\sqrt{\big(w_j^\top \Sigma_t^{(j)} w_j\big)\big(w_i^\top \Sigma_{t+1}^{(i)} w_i\big)}
~=~ \mathcal O(\varepsilon),
\quad}
\]
so $w_j^\top C w_i \to 0$ as $\varepsilon\to 0$; only within-mode blocks remain:
\begin{equation}\label{eq:block-diag}
C~\approx~\sum_{m=1}^M {q}_m^2\, C_{mm}\qquad(\text{block-diagonal approximation}).
\end{equation}
\end{proposition}

\begin{proof}[Proof sketch]
Decompose $C=\sum_{m,n}{q}_m{q}_n C_{mn}$. For any unit $w_j,w_i$,
Cauchy--Schwarz yields
$\big|w_j^\top C_{mn} w_i\big|
\le \sqrt{(w_j^\top \Sigma_t^{(m)} w_j)(w_i^\top \Sigma_{t+1}^{(n)} w_i)}$.
For $m\neq n$, apply assumption \eqref{eq:modal-sep} to obtain the $\varepsilon$ bound; keep the within-mode terms ($m=n$) as the alignment/cancellation component. Weighting by ${q}_m{q}_n$ gives \eqref{eq:cross-term-bound}. When $i\neq j$, only cross-mode terms are relevant, giving the $\mathcal O(\varepsilon)$ bound; letting $\varepsilon\to 0$ yields \eqref{eq:block-diag}.
\end{proof}
