# Supplementary material for: Less is More: Clustered Cross-Covariance Control for Offline RL
Source: arXiv:2601.20765 source file (2026-01-31)
Supplement: Supplementary file 6 [file app_MultiModal-Data.tex]

\newpage
\section{MultiModal Data}
\begin{proposition}[Block-diagonal cross-time covariance under multimodal data]\label{prop:block-diag-crosscov}
Let the offline data distribution be a mixture $D=\sum_{m=1}^M {q}_m D_m$ with ${q}_m>0$ and $\sum_m {q}_m=1$, where $D_m$ is the $m$-th mode (peak).
Define the gradient field $g_t(x):=\nabla_x Q_{\theta_t}(x)$.
For each mode, let
\[
\Sigma_t^{(m)}:=\mathrm{Var}\!\big(g_t(x)\mid x\!\in\!D_m\big),\qquad
\Sigma_{t+1}^{(m)}:=\mathrm{Var}\!\big(g_{t+1}(x)\mid x\!\in\!D_m\big),
\]
and define the cross-time, cross-mode covariance
\[
C_{mn}:=\mathrm{Cov}\!\big(g_t(x')\mid x'\!\in\!D_m,\; g_{t+1}(x)\mid x\!\in\!D_n\big).
\]
Assume there exists $\varepsilon\in[0,1)$ such that for any $m\neq n$ and any unit vectors $u,v$,
\begin{equation}\label{eq:modal-sep}
\big|u^\top C_{mn}\, v\big|
~\le~
\varepsilon\,\sqrt{\big(u^\top \Sigma_t^{(m)} u\big)\big(v^\top \Sigma_{t+1}^{(n)} v\big)}.
\end{equation}
(This captures \emph{modal separation/low similarity}: cross-mode gradient correlation is bounded by $\varepsilon\ll 1$; it is implied, e.g., by sufficiently small NTK similarity across modes.)

Let the overall cross-time covariance be
\[
C~:=~\mathrm{Cov}\!\big(g_t(x'),\,g_{t+1}(x)\big)
~=~\sum_{m,n=1}^M {q}_m{q}_n\,C_{mn}.
\]
Then for any pair of mode indices $(i,j)$ and unit directions $w_j$ (for $x'\!\in\!D_j$) and $w_i$ (for $x\!\in\!D_i$),
\begin{equation}\label{eq:cross-term-bound}
\big|\,w_j^\top C\, w_i\,\big|
~\le~
\pi_i\pi_j\,\varepsilon\,
\sqrt{\big(w_j^\top \Sigma_t^{(j)} w_j\big)\big(w_i^\top \Sigma_{t+1}^{(i)} w_i\big)}
~+~ \sum_{m=1}^M {q}_m^2\,\big|w_j^\top C_{mm} w_i\big|.
\end{equation}
In particular, when $i\neq j$ (cross-mode pairing) and $w_j,w_i$ are chosen within their respective modes,
\[
{\quad
\big|\,w_j^\top C\, w_i\,\big|
~\le~
\pi_i\pi_j\,\varepsilon\,
\sqrt{\big(w_j^\top \Sigma_t^{(j)} w_j\big)\big(w_i^\top \Sigma_{t+1}^{(i)} w_i\big)}
~=~ \mathcal O(\varepsilon),
\quad}
\]
so $w_j^\top C w_i \to 0$ as $\varepsilon\to 0$; only within-mode blocks remain:
\begin{equation}\label{eq:block-diag}
C~\approx~\sum_{m=1}^M {q}_m^2\, C_{mm}\qquad(\text{block-diagonal approximation}).
\end{equation}
\end{proposition}

\begin{proof}[Proof sketch]
Decompose $C=\sum_{m,n}{q}_m{q}_n C_{mn}$. For any unit $w_j,w_i$,
Cauchy--Schwarz yields
$\big|w_j^\top C_{mn} w_i\big|
\le \sqrt{(w_j^\top \Sigma_t^{(m)} w_j)(w_i^\top \Sigma_{t+1}^{(n)} w_i)}$.
For $m\neq n$, apply assumption \eqref{eq:modal-sep} to obtain the $\varepsilon$ bound; keep the within-mode terms ($m=n$) as the alignment/cancellation component. Weighting by ${q}_m{q}_n$ gives \eqref{eq:cross-term-bound}. When $i\neq j$, only cross-mode terms are relevant, giving the $\mathcal O(\varepsilon)$ bound; letting $\varepsilon\to 0$ yields \eqref{eq:block-diag}.
\end{proof}

% \begin{corollary}[Plugging modal directions $w_i$ into the TD-variance formula]
% In the TD variance expression of the lemma, if $x\!\in\!D_i$ and $x'\!\in\!D_j$ with $i\neq j$,
% and we choose the unit perturbation directions $w_i,w_j$ within their respective modes, then
% \[
% \mathrm{Var}[\delta_{t+1}]
% ~=~\gamma^2 k_2^2\, w_j^\top \Sigma_t^{(j)} w_j
% ~+~ k_1^2\, w_i^\top \Sigma_{t+1}^{(i)} w_i
% ~-~2\gamma k_1k_2\, w_j^\top C\, w_i
% \;\approx\;
% \gamma^2 k_2^2\, w_j^\top \Sigma_t^{(j)} w_j
% ~+~ k_1^2\, w_i^\top \Sigma_{t+1}^{(i)} w_i,
% \]
% where the last step uses Proposition~\ref{prop:block-diag-crosscov} to bound $w_j^\top C w_i=\mathcal O(\varepsilon)$.
% Under an isotropic approximation $w_m^\top\Sigma_{\cdot}^{(m)} w_m\simeq\sigma_g^2$ and $k_1,k_2$ proportional to the inter-modal distance $\|\mu_i-\mu_j\|$, we obtain
% $\mathrm{Var}[\delta_{t+1}] \propto \|\mu_i-\mu_j\|^2$.
% \end{corollary}

\newpage
\begin{lemma}[Multimodal data + unimodal policy induces interpolation; NTK yields cross-modal averaging and OOD value bias]
\label{lem:interp-ntk-bias}
Fix a state $s$. Suppose the behavior actions at $s$ follow a mixture
$d(a\mid s)=\sum_{m=1}^M \pi_m\, d_m(a\mid s)$ with $\pi_m>0$, $\sum_m\pi_m=1$, where each $d_m(\cdot\mid s)$ is unimodal with mean $\mu_m$ and bounded covariance. Consider fitting a unimodal Gaussian policy
$\pi_\theta(a\mid s)=\mathcal N(\mu_{\theta}(s),\sigma^2 I)$
by maximizing a weighted log-likelihood (AWR/BC) objective
$\max_\theta~\E_{a\sim d(\cdot\mid s)}[\,w(s,a)\,\log\pi_\theta(a\mid s)\,]$
with $w(s,a)\ge 0$. Then the optimal mean is
\[
\mu_{\theta}^{}(s)=\frac{\E_{a\sim d}[\,w(s,a)\,a\,]}{\E_{a\sim d}[\,w(s,a)\,]}
=\sum_{m=1}^M \alpha_m\, \mu_m^\wedge,\quad
\alpha_m:=\frac{\pi_m\,\E_{d_m}[w]}{\sum_\ell \pi_\ell\,\E_{d_\ell}[w]},\;\;
\mu_m^\wedge:=\frac{\E_{a\sim d_m}[\,w(s,a)\,a\,]}{\E_{a\sim d_m}[\,w(s,a)\,]},
\]
i.e., $\mu_{\theta}^{}(s)$ lies in the convex hull of modal (weighted) means. Denote this
\emph{interpolation point} by $a_{\mathrm{int}}:=\mu_{\theta}^{}(s)$.

Let $Q$ be trained from offline data $\{(s,a_i,y_i)\}_{i=1}^N$ with $a_i\in \cup_m \mathrm{supp}(d_m)$ and targets $y_i$ (e.g., TD targets), using kernel ridge regression under the NTK linearization with kernel $\Theta$. Write $K$ for the $N{\times}N$ kernel matrix and $k_\ast$ for the kernel vector at $(s,a_{\mathrm{int}})$. Assume:
(i) \textbf{Block-diagonal dominance:} after reordering by modes, $K=\mathrm{diag}(K_{11},\dots,K_{MM})+E$ with $\|E\|_\mathrm{op}\le \varepsilon \min_m \lambda_{\min}(K_{mm})$ for some $\varepsilon\in[0,1)$;
(ii) \textbf{Within-mode concentration:} for each $m$, $k_\ast$ is approximately constant on the $m$-th block and the targets are tight in that block, i.e., 
$\max_{i\in m}|k_{\ast i}-\bar k_m|\le \eta_k \bar k_m$ and 
$\frac{1}{n_m}\sum_{i\in m}|y_i-\bar y_m|\le \eta_y$, where $\bar k_m$ and $\bar y_m$ are block means;
(iii) ridge parameter $\lambda\ge 0$ is small.

Then there exist weights $\beta_m\ge 0$, $\sum_m \beta_m=1$, depending on $(k_\ast,K)$, such that the NTK predictor at the interpolation point satisfies
\[
\widehat Q(s,a_{\mathrm{int}})\;=\;\sum_{m=1}^M \beta_m\,\bar y_m \;+\; \mathcal O(\varepsilon+\eta_k+\eta_y+\lambda).
\]
In particular, if the mode-wise target means differ (let $\Delta_Q:=\max_{m,n}|\bar y_m-\bar y_n|>0$) and the true value $Q^\pi(s,a_{\mathrm{int}})$ is \emph{not equal} to the convex combination $\sum_m \beta_m \bar y_m$ (which is generic in low-density bridges between modes), then the OOD prediction bias obeys
\[
\big|\widehat Q(s,a_{\mathrm{int}})-Q^\pi(s,a_{\mathrm{int}})\big|
\;\ge\;
\big|\,\sum_m \beta_m \bar y_m - Q^\pi(s,a_{\mathrm{int}})\,\big|
\;-\; \mathcal O(\varepsilon+\eta_k+\eta_y+\lambda),
\]
i.e., the NTK estimator \emph{cross-modally averages} modal targets at the policy’s interpolation point, yielding systematic OOD error unless $Q^\pi$ happens to match that average along the low-density region.
\end{lemma}

\begin{proof}[Proof sketch]
(A) \emph{Policy interpolation.} For fixed $\sigma^2$, maximizing $\E[w\log\pi]$ is equivalent to minimizing $\E[w\|a-\mu\|^2]$, 
whose minimizer is the weighted mean $\mu_{\theta}^{}(s)$; 
decomposing by modes yields the convex combination above. 
Hence sampling from $\mathcal N(\mu_{\theta}^{}(s),\sigma^2 I)$ puts nonzero mass in low-density regions between separated modes.

(B) \emph{NTK cross-modal averaging.} Under block-diagonal dominance and within-mode concentration, the kernel ridge solution
$\widehat Q(x_\ast)=k_\ast^\top(K+\lambda I)^{-1}y$
reduces (up to $\mathcal O(\varepsilon+\eta_k+\lambda)$) to a sum of block-wise scalars times block-wise target averages, giving the stated convex combination with coefficients $\beta_m$ proportional to the effective kernel mass of $x_\ast$ toward each block. Tightness of targets within blocks contributes $\mathcal O(\eta_y)$.
\end{proof}
