# Supplementary material for: Less is More: Clustered Cross-Covariance Control for Offline RL
Source: arXiv:2601.20765 source file (2026-01-31)
Supplement: Supplementary file 7 [file locomotion-table.tex]

\subsection{Main result}

In the reduced-size regime of D4RL MuJoCo with only 10k trajectories per task we compare TD3+BC, BC, CQL, IQL, DOGE, TSRL, and Ours and report mean normalized scores with standard deviations as shown in the table overall Ours attains the best results on nearly all tasks and achieves the highest overall average of 75.7 clearly ahead of TSRL at 57.2 and other offline RL baselines yielding about 29.7 points over CQL about 25.0 over DOGE and about 44.2 over TD3+BC across Hopper Halfcheetah Walker2d and Ant variants the advantage of Ours is consistent indicating better data efficiency and robust generalization under the same sample budget.

\begin{figure}[h]
	\centering
    \subfigure{\label{fig:gym-halfcheetah}\includegraphics[width=0.23\textwidth]{./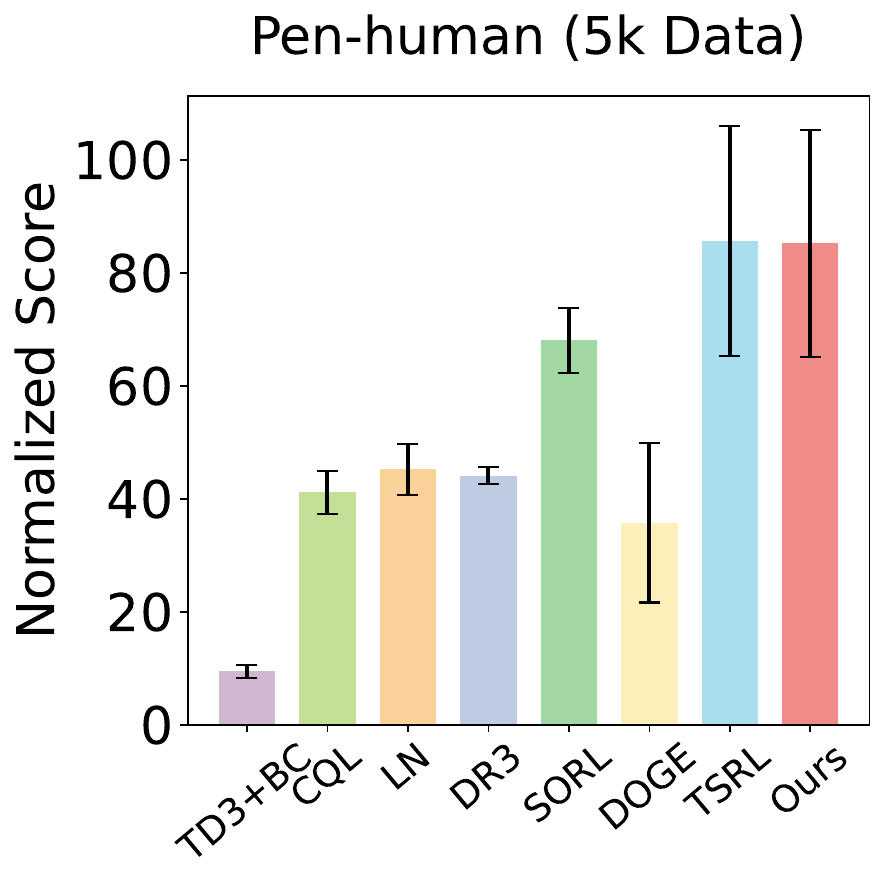}}
    % \hspace{0.02\textwidth}
    \subfigure{\label{fig:gym-hopper}\includegraphics[width=0.23\textwidth]{./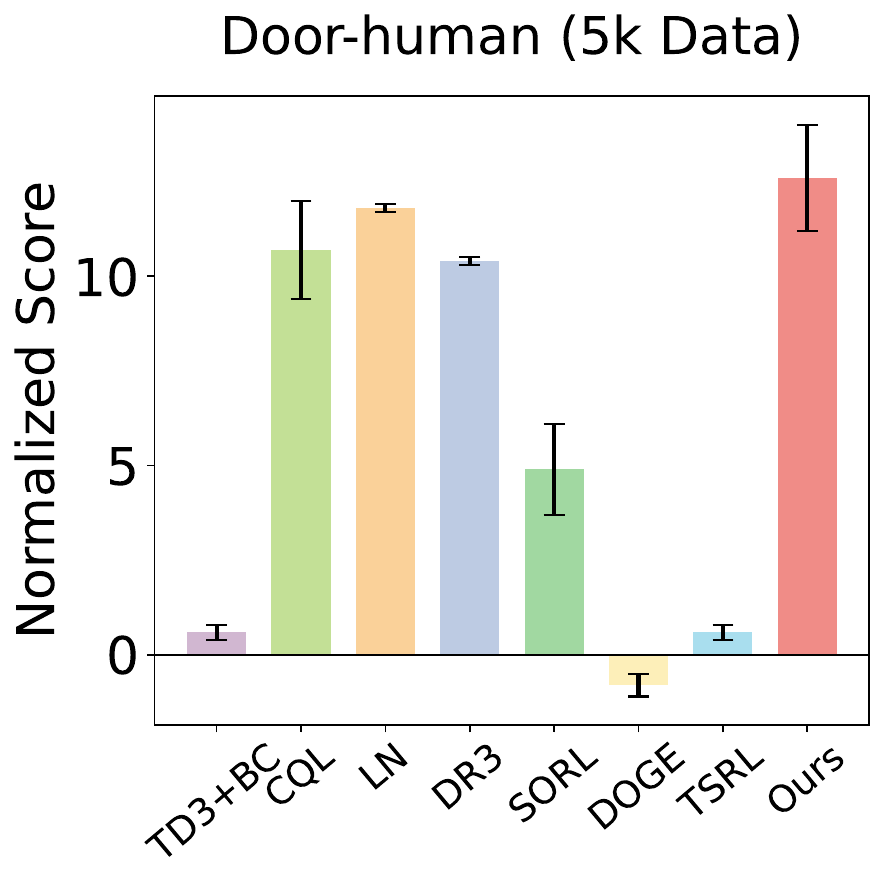}}
    % \hspace{0.02\textwidth}
    \subfigure{\label{fig:gym-walker2d}\includegraphics[width=0.23\textwidth]{./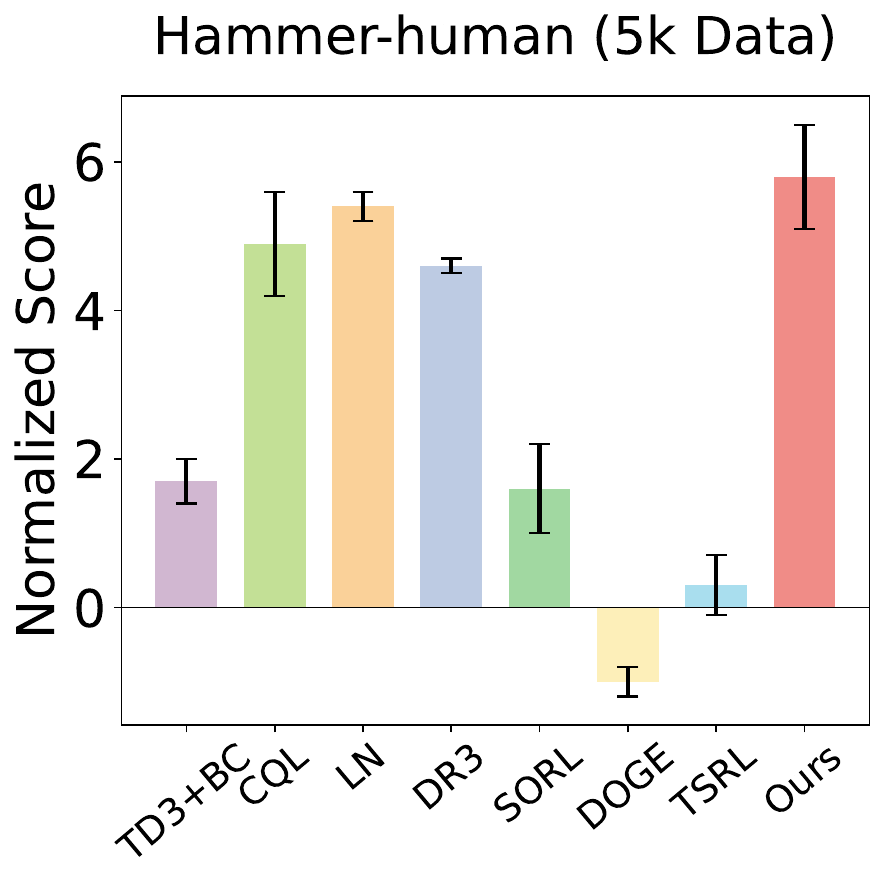}}
    % \hspace{0.02\textwidth}
    \subfigure{\label{fig:gym-ant}\includegraphics[width=0.23\textwidth]{./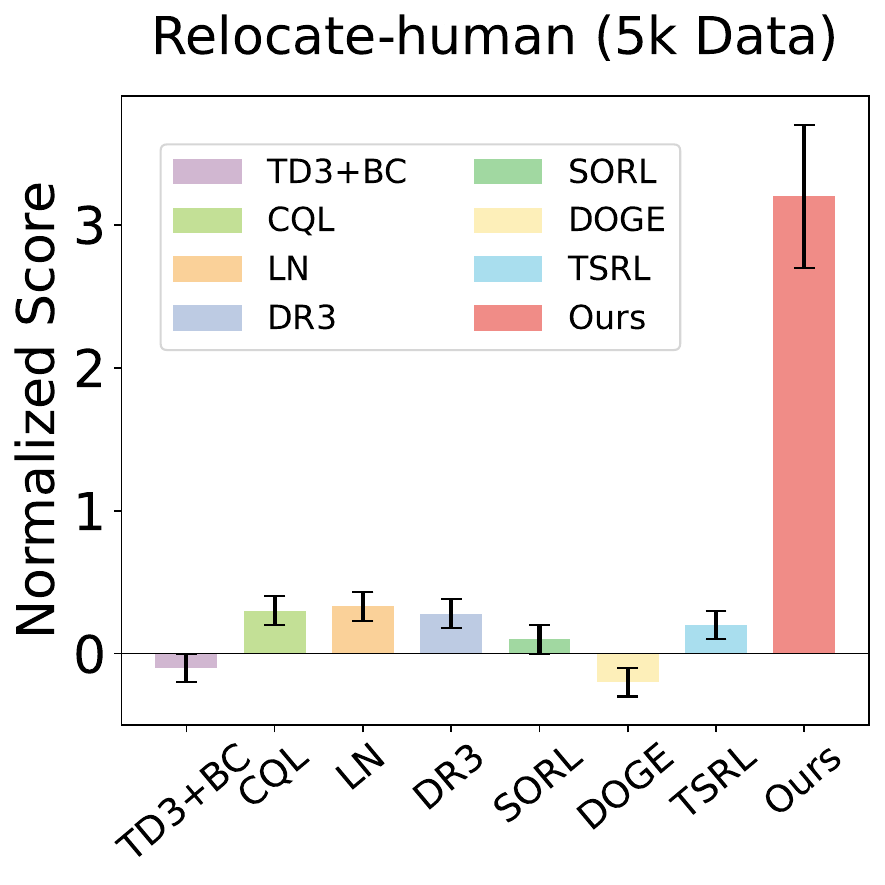}}    
\caption{Comparison on gym Adroit tasks over different methods.} 
% \vspace{-2em}
\label{fig:human}
\end{figure}

\begin{table}[t]
\centering
\caption{Normalized score on gym locomotion tasks with reduced-size datasets (10k).
-full-replay, -medium-replay and -medium-expert is abbreviated to fr, mr and me., respectively.
}
\resizebox{\textwidth}{!}{
\begin{tabular}{lccccccc}
\toprule
Task & TD3+BC & BC & CQL & IQL & DOGE & TSRL & Ours \\
\midrule
Hopper-m       & 30.7$\pm$13.2 & 28.8$\pm$12.7 & 50.1$\pm$22.3 & 61.0$\pm$6.2  & 55.6$\pm$8.3  & 60.9$\pm$4.1   & \textbf{69.2$\pm$12.7} \\
Hopper-mr      & 11.3$\pm$4.7  & 19.7$\pm$18.8 & 13.2$\pm$2.0  & 16.2$\pm$3.0  & 19.1$\pm$3.3  & 23.5$\pm$8.8   & \textbf{45.9$\pm$8.4} \\
Hopper-me      & 22.6$\pm$13.9 & 38.2$\pm$8.7  & 43.2$\pm$6.9  & 51.7$\pm$7.0  & 36.8$\pm$34.5 & 56.6$\pm$13.9  & \textbf{81.3$\pm$6.0} \\
Hopper-e       & 53.6$\pm$17.1 & 50.3$\pm$9.5  & 56.1$\pm$26.4 & 60.9$\pm$9.6  & 62.2$\pm$21.7 & 76.7$\pm$20.4  & \textbf{107.0$\pm$2.8} \\
Hopper-fr      & 32.0$\pm$13.5 & 30.5$\pm$12.4 & 45.0$\pm$22.0 & 56.0$\pm$6.3  & 54.0$\pm$8.4  & 53.4$\pm$11.3  & \textbf{65.3$\pm$9.4} \\
\midrule
Halfcheetah-m  & 25.9$\pm$8.4  & 40.2$\pm$8.0  & 41.7$\pm$2.2  & 35.6$\pm$2.9  & 42.8$\pm$2.9  & 43.3$\pm$2.8   & \textbf{46.3$\pm$3.1} \\
Halfcheetah-mr & 29.1$\pm$8.3  & 25.2$\pm$8.8  & 16.3$\pm$4.9  & 34.1$\pm$6.3  & 26.3$\pm$3.1  & 27.7$\pm$3.8   & \textbf{43.1$\pm$5.3} \\
Halfcheetah-me & 23.5$\pm$13.6 & 33.7$\pm$7.4  & 39.7$\pm$6.4  & 14.3$\pm$7.3  & 33.1$\pm$8.8  & 37.2$\pm$14.9  & \textbf{46.0$\pm$3.5} \\
Halfcheetah-e  & 26.4$\pm$4.2  & 25.8$\pm$3.4  & 5.8$\pm$1.3   & -1.1$\pm$3.8  & 1.4$\pm$3.1   & 42.0$\pm$26.4  & \textbf{75.8$\pm$5.2} \\
Halfcheetah-fr & 28.0$\pm$8.6  & 41.0$\pm$8.1  & 45.0$\pm$2.4  & 33.0$\pm$3.0  & 43.0$\pm$3.1  & 41.0$\pm$3.0   & \textbf{58.1$\pm$3.4} \\
\midrule
Walker2d-m     & 11.2$\pm$19.2 & 25.4$\pm$8.6  & 54.1$\pm$15.5 & 34.2$\pm$5.2  & 53.7$\pm$12.6 & 47.3$\pm$10.1  & \textbf{65.9$\pm$7.8} \\
Walker2d-mr    & 9.3$\pm$6.6   & 2.5$\pm$2.8   & 13.8$\pm$5.3  & 17.7$\pm$8.9  & 15.5$\pm$9.2  & 27.6$\pm$12.4  & \textbf{55.4$\pm$5.9} \\
Walker2d-me    & 12.4$\pm$15.7 & 35.1$\pm$14.4 & 26.0$\pm$14.0 & 38.0$\pm$12.2 & 42.5$\pm$11.4 & 50.9$\pm$26.4  & \textbf{96.3$\pm$10.4} \\
Walker2d-e     & 29.5$\pm$23.5 & 37.9$\pm$6.3  & 56.0$\pm$29.4 & 16.2$\pm$3.2  & 81.2$\pm$18.6 & 104.9$\pm$10.6 & \textbf{109.5$\pm$0.3} \\
Walker2d-fr    & 14.2$\pm$19.5 & 26.2$\pm$8.7  & 55.0$\pm$16.0 & 36.0$\pm$5.6  & 55.5$\pm$12.3 & 44.3$\pm$10.4  & \textbf{77.3$\pm$7.1} \\
\midrule
Ant-me         & 52.0$\pm$18.2 & 36.0$\pm$9.0  & 74.0$\pm$25.0 & 66.0$\pm$10.5 & 82.0$\pm$16.4 & 83.6$\pm$12.4  & \textbf{100.9$\pm$5.0} \\
Ant-m          & 46.0$\pm$17.4 & 33.0$\pm$8.2  & 62.0$\pm$22.1 & 56.0$\pm$9.3  & 69.0$\pm$15.2 & 72.2$\pm$10.6  & \textbf{84.5$\pm$6.1} \\
Ant-mr         & 31.0$\pm$15.5 & 21.0$\pm$7.3  & 36.0$\pm$16.3 & 41.0$\pm$10.8 & 46.0$\pm$12.9 & 49.4$\pm$13.1  & \textbf{65.8$\pm$6.9} \\
Ant-e          & 72.0$\pm$25.0 & 57.0$\pm$14.2 & 94.0$\pm$29.4 & 82.0$\pm$15.0 & 98.0$\pm$20.3 & 100.7$\pm$12.6 & \textbf{109.6$\pm$2.7} \\
Ant-fr         & 70.0$\pm$24.0 & 55.0$\pm$9.5  & 92.0$\pm$26.5 & 80.0$\pm$15.0 & 96.0$\pm$20.0 & 99.8$\pm$12.0  & \textbf{107.6$\pm$3.2} \\
\midrule
Average & 31.5 & 33.1 & 46.0 & 41.4 & 50.7 & 57.2 & 75.7 \\
\bottomrule
\end{tabular}}
\end{table}
