# Supplementary material for: Less is More: Clustered Cross-Covariance Control for Offline RL
Source: arXiv:2601.20765 source file (2026-01-31)
Supplement: Supplementary file 8 [file appendix.tex]

\section{Some Possibilities}
\subsection{MoE for RL}
\paragraph{Learning the routing}
	The proposed method follows the typical setting of MOE method, which decomposes a complex policy $\pi$ into a mixture of low-level stochastic policies with each of them as a probability distribution, represented as the following: 
	\begin{align}
	\label{eq:mixture_define}
    	\pi_{\{\theta, \psi\}}(a_{t}|s_{t}) &= \sum_{i=1}^{K} w_{\theta_{i}}(s_{t}) \pi_{\psi_{i}}(a_{t}|s_{t}), \\ &s.t.\, \sum_{i=1}^{K}w_{\theta_{i}} = 1, \, w_{\theta_{i}}>0,
	\end{align}
	where each $\pi_{\psi_{i}}$ denotes the action distribution within each low-level policy, \emph{i.e.} a \textit{actor}, and $K$ denotes the number of actors. $w_{\theta_{i}}$ is the weight that specifies the probability of the activating actor $\pi_{\psi_i}$, which is called the \textit{routing} function. According to the GMM assumption~\cite{PRML}, $w_{\theta}$ is a Categorical distribution and $\pi_{\psi}$ is a unimodal Gaussian distribution. For $\forall  i \in \{1,2,...,K\}$, $\theta_i$ and $\psi_i$ are parameters of $w_{\theta_i}$ and $\pi_{\psi_i}$, respectively. %Usually, 
	After the policy decomposition with MOE method, we can rewrite the update rule as:
	\begin{equation}
		\begin{aligned}
			\theta \leftarrow \theta + \nabla_{\theta}\mathbb{E}_{a_t\sim\pi_{\{\theta, \psi\}}(a_{t}|s_{t})}[Q_{\phi}(s_t, a_t)],\\
			\psi \leftarrow \psi + \nabla_{\psi}\mathbb{E}_{a_t\sim\pi_{\{\theta, \psi\}}(a_{t}|s_{t})}[Q_{\phi}(s_t, a_t)].
		\end{aligned}
	\end{equation}
	In practice, if we apply a Gaussian distribution for each of the low-level policies here in PMOE, the overall MoE will end up to be a GMM. However, sampling from the mixture distributions of actors $\pi_{\{\theta, \psi\}}(a_t|s_t)$ embeds a sampling process from the categorical distribution $w_{\theta}$, which makes the differential calculation of policy gradients commonly applied in DRL hard to achieve. We provide a theoretically guaranteed solution for approximating the gradients in the sampling process of MoE and apply it for optimising the MoE policy model within DRL, which will be described in details.

    The routing function in MOE typically involves a sampling process from a categorical distribution (due to the discontinuity among multiple experts), which is indifferentiable~\cite{gumbel}. To handle this difficulty, we propose a new gradient estimator for this routing function. 
	
% 	Since the network parameter $\theta_k$ is updated by the gradient based algorithm, we should estimate the proper gradient update direction for $\theta_k$.
	Specifically, given a state $s_t$, we sample one action $a_t^i$ from each actor $\pi_{\psi_{i}}$, to get a total of $K$ actions  $\{a_t^i; i=1, 2,\cdots, K\}$, and compute $K$ Q-value estimations $\{Q_{\phi}(s_t, a_t^i); i=1, 2,\cdots, K\}$ for each of the actions. We say the actor $j$ is the “optimal" actor under the Q-value estimation if $j = \arg\max_i Q_{\phi}(s_t, a_t^i)$.
	There exists a frequency of the actor $j$ to be the “optimal" actor given a set of state $\{s_t\}$, here we propose a new gradient estimator which optimise $\theta_k$ towards the frequency.
	\begin{proposition}
    \textit{Frequency Approximate Gradient} For a stochastic mixture-of-experts, the gradient value of a single-instance sampling process for the routing function $w_\theta$ can be estimated with the frequency approximate gradient, which is defined as:
		\begin{equation}
		\text{grad} = \delta_k\nabla_{\theta_k}w_{\theta_k}, \,\delta_k = -\mathbbm{1}_k^{\text{best}} + w_{\theta_k},
	\end{equation}
		where $\nabla_{\theta_k}w_{\theta_k}$ is the gradient of $w_{\theta_k}$ for parameters $\theta_k$ and $\mathbbm{1}_k^{\text{best}}$ is the indicator function that $\mathbbm{1}_k^{\text{best}} = 1$ if $k = \arg\max_jQ_{\phi}(s_{t}, a_{t}^j)$ and $\mathbbm{1}_k^{\text{best}} = 0$ otherwise.
	\end{proposition}

    Then $\theta_k$ is updated via a gradient descent based algorithm, \emph{e.g.}, Stochastic Gradient Descent (SGD):
	\begin{equation}
		\theta_k \leftarrow \theta_k - \delta_k\nabla_{\theta_k}w_{\theta_k}.
	\end{equation}
	
	% According to the formation of Eq~\eqref{eq:lead_to_freq_loss}, 
    We can build an elegant loss function that achieves the same goal of gradient estimating:
	\begin{equation}
	\label{eq:freq_loss}
	\mathcal{L}_{freq} = (v-w)(v-w)^T, w=[w_{\theta_{1}}, w_{\theta_{2}}, \cdots, w_{\theta_{K}}],
	\end{equation}
	$v$ is a one-hot code vector $v = [v_1, v_2, \cdots, v_K]$ with:
	\begin{equation}
		\label{eq:compute_v}
		v_j = \left\{
		\begin{aligned}
		&1, \,\text{if}\, j=\arg\max_{i}Q_{\phi}(s_t, a_t^i);\\
		&0, \,\text{otherwise}.
		\end{aligned}
		\right.
	\end{equation}
    
	\paragraph{Learning the Actor}
	\label{sec:actor_loss}
	To update the $\psi_i$ within each actor, we provide two approaches of optimising the actors: \textit{back-propagation-all} and \textit{back-propagation-max} manners. 

	For the \textit{back-propagation-all} approach, we update all the actor:
	\begin{equation}
	\mathcal{L}_{pri}^{bpa} = -\sum_i^KQ_{\phi}(s_{t}, a_{t}^i), \, a_{t}^i \sim \pi_{\psi_{i}}(a_t|s_t).
	\end{equation}
	
	For the \textit{back-propagation-max} approach, 
	we use the highest Q-value estimation as the actor loss:
	\begin{equation}
	\label{eq:pri_loss}
	\mathcal{L}_{pri}^{bpm} = -\max_{i=1, 2, \cdots, K}\{Q_{\phi}(s_{t}, a_{t}^i)\}, \, a_{t}^i \sim \pi_{\psi_{i}}(a_t|s_t).
	\end{equation}
	\label{sec:backprog_all}
	
	With either approach, we have the same stochastic policy gradients as following:
	\begin{equation}
	\begin{aligned}
		\nabla_{\psi_{i}}\mathcal{L}_{pri} 
		=& -\nabla_{\psi_j} \mathbb{E}_{\pi_{\psi_i}}[Q_{\phi}(s_{t}, a_{t})]\\
		=& \mathbb{E}_{\pi_{\psi_i}}[-Q_{\phi}(s_{t}, a_{t})\nabla_{\psi_j}\log\pi_{\psi_j}(a_t|s_t)]
	\end{aligned}
	\end{equation}

	Ideally, both approaches are feasible for learning a MoE model. However, in practice, we find that the \textit{back-propagation-all} approach will tend to learn actors that are close to each other, while the \textit{back-propagation-max} approach is capable of keeping actors distinguishable. The phenomenon is demonstrated in our experimental analysis. Therefore, we adopt the \textit{back-propagation-max} approach as the default setting of MoE model without additional clarification.

	\paragraph{Learning the Critic}
	\label{sec:critic_loss}
	Similar to the standard off-policy RL algorithms, our Q-value network is also trained to minimise the Bellman residual:
	\begin{equation}
    	\begin{aligned}
    	\mathcal{L}_{critic} = &\mathbb{E}_{(s_t, a_t)\sim\mathcal{D}} [\|Q_{\phi}(s_t, a_t) - [r_t + \\ &\gamma \max_{a_{t+1}}Q_{\bar{\phi}}(s_{t+1}, a_{t+1})]\|_2], a_{t+1}  + R(CQL) \sim \pi(a_{t+1}|s_{t+1})
    	\end{aligned}
		\label{eq:critic_loss}
	\end{equation}
	where $\bar{\phi}$ is the parameters of the target network.

	The learning component can be easily embedded into the popular actor-critic algorithms, such as soft actor-critic (CQL), one of the state-of-the-art offline RL algorithms.
    % In SAC, $Q_{\psi}(s_t, a_t^j)$ is substituted with $Q_{\psi}(s_t, a_t^j) + \alpha\mathcal{H}_j$, where $\alpha$ is temperature and $\mathcal{H}_j = -\log\pi_{\psi_{j}}(a_t|s_t)$ is the entropy which are the same as in SAC. The algorithm is summarised in Algorithm~\ref{alg:training}. When $K=1$, our algorithm simply reduces to the standard SAC. 

    \begin{algorithm}[]
    \caption{MOE for RL with Multiple Datasets}
    \label{alg:training}
 \begin{algorithmic}
    \STATE {\bfseries Input:} 
    $\theta,
    % $\{\theta_i\}_{i=1}^K,
    \{\psi_i\}_{i=1}^K, \{\phi_i\}_{i=1}^K$
    % \STATE Initialise target networks $\{\bar{\theta}_i\leftarrow\theta_i\}_{i=1}^K, \{\bar{\psi}_i\leftarrow\psi_i\}_{i=1}^K, \{\bar{\phi}_i\leftarrow\phi_i\}_{i=1}^K$
    \STATE {Split K datasets: $\{\mathcal{D}_i\}_{i=1}^K$ from dataset $\mathcal{D}$}
    
    \REPEAT
        \FOR{each dataset $\mathcal{D}_i$ where $i \in \{1,...,K\}$}
            \FOR{each update step}
                \STATE {Sample from: $\{s_t, a_t, s_{t+1}, r_t\} \sim \mathcal{D}_i$}
                \STATE {Compute $\mathcal{L}_{freq}$ with Eq. \eqref{eq:freq_loss}}
                \STATE {Compute $\mathcal{L}_{pri}^i$ with Eq.~\eqref{eq:pri_loss}}
                \STATE {Compute $\mathcal{L}_{critic}^i$ with Eq.~\eqref{eq:critic_loss}}
                \STATE {Update policy $i$ with: \\
                $\theta \leftarrow \theta - \lambda_\theta\nabla_{\theta}\mathcal{L}_{freq}$, $\psi_i \leftarrow \psi_i - \lambda_\psi\nabla_{\psi_i}\mathcal{L}_{pri}^i$}
                
                \STATE {Update critic $i$ with: \\
                $\phi_i \leftarrow \phi_i - \lambda_\phi\nabla_{\phi_i}\mathcal{L}_{critic}^i$}
            \ENDFOR
        \ENDFOR
    \UNTIL{converge}
    
    \STATE {\bfseries Output:} $\{\theta_i\}_{i=1}^K, \{\psi_i\}_{i=1}^K, \{\phi_i\}_{i=1}^K.$
 \end{algorithmic}
\end{algorithm}

\begin{table}[h]
\caption{Complete results on D4RL locomotion tasks with our method's performance}
\scriptsize

\begin{adjustbox}{center}
\begin{tabular}{cccccccccc}
\toprule
\textbf{Task}   & \textbf{Size}    & \textbf{BC}           & \textbf{TD3+BC}           & \textbf{MOPO} & \textbf{CQL}  & \textbf{IQL}& \textbf{DOGE}& \textbf{TSRL}  & \textbf{ours}     \\ 
\midrule
Hopper-m        & 10k       & 29.7$\pm$11.7          & 45.1$\pm$18.6 & 5.5$\pm$2.3   & 43.1$\pm$24.6 &46.7$\pm$6.5           & 44.2 $\pm$ 10.2          & {62.0$\pm$3.7}       & \textbf{67.24}       \\ 
Hopper-mr       & 10k       & 12.1$\pm$5.3           & 7.3$\pm$6.1  & 6.8$\pm$0.3   & 2.3$\pm$1.9   & 13.4$\pm$3.1           & 17.9 $\pm$ 4.5           & {21.8$\pm$8.2}     & \textbf{74.65}   \\ 
Hopper-me       & 10k       & 27.8$\pm$10.7         & 17.8$\pm$7.9  & 5.8$\pm$5.8   & 29.9$\pm$4.5   & 34.3$\pm$8.7          & 50.5 $\pm$ 25.2          & {50.9$\pm$8.6} & \textbf{65.11}  \\ 
Hopper-e        & 10k       & 20.8$\pm$6.9          &23.2$\pm$18.2  &6.5$\pm$3.7    & 33.0$\pm$22.2 &38.4$\pm$11.3           & 54.5$\pm$21.5 & {82.7$\pm$21.9}  &\textbf{105.10}    \\
Halfcheetah-m   & 10k       & 26.4$\pm$7.3          & 16.4$\pm$10.2 & -1.1$\pm$4.1  & 35.8$\pm$3.8  & 29.9$\pm$0.12          &  36.2$\pm$3.4         & {38.4$\pm$3.1}   & \textbf{47.43}     \\ 
Halfcheetah-mr  & 10k       & 14.3$\pm$7.8          & 17.9$\pm$9.5  &11.7$\pm$5.2   &8.1$\pm$9.4   &22.7$\pm$6.4 &  23.4$\pm$3.6          & {28.1$\pm$3.5}     & \textbf{42.85}    \\ 
Halfcheetah-me  & 10k       & 19.1$\pm$9.4         &15.4$\pm$10.7  &-1.1$\pm$1.4   & 26.5$\pm$10.8 &10.5$\pm$8.8 &  26.7$\pm$6.6          & {39.9$\pm$21.1}  & \textbf{50.24}  \\ 
Halfcheetah-e   & 10k       & 1.10$\pm$2.4          & 1.72$\pm$3.3  &-0.6$\pm$1.1   &4.2$\pm$0.94   &-2.0$\pm$0.4&   1.4$\pm$2.1        &  {40.6$\pm$24.4}   &\textbf{68.26} \\ 
Walker2d-m      & 10k       & 15.8$\pm$14.1         & 7.4$\pm$13.1  &3.1$\pm4.7$    &18.8$\pm$18.8  &22.5$\pm$3.8&   45.1 $\pm$ 10.2         & {49.7$\pm$10.6}    & \textbf{61.52}      \\ 
Walker2d-mr     & 10k       & 1.4$\pm$1.9           &5.7$\pm$5.8    &3.3$\pm$2.7    &8.5$\pm$2.19   &10.7$\pm$11.9           &  13.5$\pm$ 8.4           &{26.0$\pm$11.3}   & \textbf{62.51}    \\ 
Walker2d-me     & 10k       & 21.7$\pm$8.2          & 7.9$\pm$9.1 &0.6$\pm$2.7    &19.1$\pm$14.4    &26.5$\pm$8.6&  35.3 $\pm$ 11.6         & {46.4$\pm$17.4}    & \textbf{63.60}   \\ 
Walker2d-e      & 10k       & 10.4$\pm$5.3          & 23.8$\pm$16.0  &1.4$\pm$3.4    &41.6$\pm$21.6  &12.6$\pm$4.5           &  72.1 $\pm$16.2           &  {102.2$\pm$11.3} &  \textbf{109} \\
\bottomrule
\end{tabular}
\end{adjustbox}  
\end{table}

\begin{table}[h]
\caption{Complete results on D4RL locomotion tasks with our method variants}
\scriptsize

\begin{adjustbox}{center}
\begin{tabular}{ccccccccccccc}
\toprule
\textbf{Task}   & \textbf{Size} & \textbf{BC} & \textbf{TD3+BC} & \textbf{MOPO} & \textbf{CQL} & \textbf{IQL} & \textbf{DOGE} & \textbf{TSRL} & \textbf{ours-cl} & \textbf{ours-fl} & \textbf{ours-moe} \\ 
\midrule
Hopper-m        & 10k & 29.7$\pm$11.7 & 40.1$\pm$18.6 & 5.5$\pm$2.3 & 43.1$\pm$24.6 & 46.7$\pm$6.5 & 44.2$\pm$10.2 & 62.0$\pm$3.7 & 58.3$\pm$5.2 & 63.1$\pm$4.8 & \textbf{67.24} \\ 
Hopper-mr       & 10k & 12.1$\pm$5.3 & 7.3$\pm$6.1 & 6.8$\pm$0.3 & 2.3$\pm$1.9 & 13.4$\pm$3.1 & 17.9$\pm$4.5 & 21.8$\pm$8.2 & 65.4$\pm$7.3 & 68.9$\pm$6.1 & \textbf{74.65} \\ 
Hopper-me       & 10k & 27.8$\pm$10.7 & 17.8$\pm$7.9 & 5.8$\pm$5.8 & 29.9$\pm$4.5 & 34.3$\pm$8.7 & 50.5$\pm$25.2 & 50.9$\pm$8.6 & 55.2$\pm$9.4 & 58.7$\pm$7.5 & \textbf{65.11} \\ 
Hopper-e        & 10k & 20.8$\pm$6.9 & 23.2$\pm$18.2 & 6.5$\pm$3.7 & 33.0$\pm$22.2 & 38.4$\pm$11.3 & 54.5$\pm$21.5 & 82.7$\pm$21.9 & 102.4$\pm$18.6 & 98.3$\pm$15.2 & \textbf{105.10} \\
Halfcheetah-m   & 10k & 26.4$\pm$7.3 & 16.4$\pm$10.2 & -1.1$\pm$4.1 & 35.8$\pm$3.8 & 29.9$\pm$0.12 & 36.2$\pm$3.4 & 38.4$\pm$3.1 & 40.2$\pm$4.3 & 43.1$\pm$3.9 & \textbf{47.43} \\ 
Halfcheetah-mr  & 10k & 14.3$\pm$7.8 & 17.9$\pm$9.5 & 11.7$\pm$5.2 & 8.1$\pm$9.4 & 22.7$\pm$6.4 & 23.4$\pm$3.6 & 28.1$\pm$3.5 & 36.8$\pm$5.7 & 39.2$\pm$4.8 & \textbf{42.85} \\ 
Halfcheetah-me  & 10k & 19.1$\pm$9.4 & 15.4$\pm$10.7 & -1.1$\pm$1.4 & 26.5$\pm$10.8 & 10.5$\pm$8.8 & 26.7$\pm$6.6 & 39.9$\pm$21.1 & 42.3$\pm$18.7 & 46.1$\pm$15.3 & \textbf{50.24} \\ 
Halfcheetah-e   & 10k & 1.10$\pm$2.4 & 1.72$\pm$3.3 & -0.6$\pm$1.1 & 4.2$\pm$0.94 & -2.0$\pm$0.4 & 1.4$\pm$2.1 & 40.6$\pm$24.4 & 55.8$\pm$20.2 & 62.4$\pm$18.7 & \textbf{68.26} \\ 
Walker2d-m      & 10k & 15.8$\pm$14.1 & 7.4$\pm$13.1 & 3.1$\pm$4.7 & 18.8$\pm$18.8 & 22.5$\pm$3.8 & 45.1$\pm$10.2 & 49.7$\pm$10.6 & 54.3$\pm$9.1 & 57.8$\pm$8.4 & \textbf{61.52} \\ 
Walker2d-mr     & 10k & 1.4$\pm$1.9 & 5.7$\pm$5.8 & 3.3$\pm$2.7 & 8.5$\pm$2.19 & 10.7$\pm$11.9 & 13.5$\pm$8.4 & 26.0$\pm$11.3 & 55.7$\pm$10.8 & 58.9$\pm$9.6 & \textbf{62.51} \\ 
Walker2d-me     & 10k & 21.7$\pm$8.2 & 7.9$\pm$9.1 & 0.6$\pm$2.7 & 19.1$\pm$14.4 & 26.5$\pm$8.6 & 35.3$\pm$11.6 & 46.4$\pm$17.4 & 55.2$\pm$15.3 & 59.8$\pm$13.7 & \textbf{63.60} \\ 
Walker2d-e      & 10k & 10.4$\pm$5.3 & 23.8$\pm$16.0 & 1.4$\pm$3.4 & 41.6$\pm$21.6 & 12.6$\pm$4.5 & 72.1$\pm$16.2 & 102.2$\pm$11.3 & 98.7$\pm$12.5 & 104.5$\pm$10.8 & \textbf{109.00} \\
\bottomrule
\end{tabular}
\end{adjustbox}  
\end{table}

\begin{table}[h]
\caption{Complete results on D4RL Adroit tasks with our method's performance}
\scriptsize

\begin{adjustbox}{center}
\begin{tabular}{cccccccccc}
\toprule
\textbf{Task}   & \textbf{Size}    & \textbf{BC}           & \textbf{TD3+BC}           & \textbf{MOPO} & \textbf{CQL}  & \textbf{IQL}& \textbf{DOGE}& \textbf{TSRL}  & \textbf{ours}     \\ 
\midrule
Pen-human       & 5k       & 34.4          & 8.4 & 9.7   & 37.5 & 71.5$\pm$5.2           & 42.6 $\pm$ 16.3          & 80.1$\pm$18.1       & \textbf{85.3$\pm$2.1}       \\
Hammer-human    & 5k       & 1.5          & 2.0 & 0.2   & 4.4 & 1.4$\pm$0.5           & -1.2 $\pm$ 0.2          & 0.2$\pm$0.3       & \textbf{5.8$\pm$0.7}       \\
Door-human      & 5k       & 0.5          & 0.5 & -0.2   & 9.9 & 4.3$\pm$1.1           & -1.1 $\pm$ 0.2          & 0.5$\pm$0.3       & \textbf{12.6$\pm$1.4}       \\
Relocate-human  & 5k       & 0.0          & -0.3 & -0.2   & 0.2 & 0.1$\pm$0.1           & -0.3 $\pm$ 0.5          & 0.1$\pm$0.1       & \textbf{3.2$\pm$0.5}       \\
Pen-cloned       & 10k      & 37.4$\pm$37.6    & -0.1$\pm$6.9    & -0.1$\pm$0.1    & 1.5$\pm$4.8  & 35.9$\pm$24.7  & 30.1$\pm$19.7    & 41.6$\pm$27.5    & \textbf{58.2$\pm$3.1}    \\
Hammer-cloned    & 10k      & 0.2$\pm$0.4      & 0.1$\pm$0.1     & 0.2$\pm$0.1     & 0.4$\pm$0.2    & 0.6$\pm$0.3     & -0.3$\pm$0.1   & 0.3$\pm$0.1            & \textbf{3.5$\pm$0.9}     \\
Door-cloned      & 10k      & -0.1             & -0.3$\pm$0.1   & -0.2$\pm$0.1   & -0.5$\pm$0.8  & -0.5$\pm$0.5   & -0.1$\pm$0.1   & 0.0$\pm$0.1                 & \textbf{2.8$\pm$1.2}     \\
Relocate-cloned  & 10k      & -0.3$\pm$0.1     & -0.3$\pm$0.1   & -0.1$\pm$0.5   & -0.2$\pm$0.1  & -0.2$\pm$0.1    & 0.0$\pm$0.1    & -0.3$\pm$0.1           & \textbf{1.4$\pm$0.7}     \\
\bottomrule
\end{tabular}
\end{adjustbox}
\label{tab:d4rl_results}
\end{table}

\begin{table}[h]
\caption{Complete results on D4RL Antmaze tasks with our method's performance}
\scriptsize

\begin{adjustbox}{center}
\begin{tabular}{cccccccccc}
\toprule
\textbf{Task}       & \textbf{Size}    & \textbf{BC}           & \textbf{TD3+BC}       & \textbf{MOPO}     & \textbf{CQL}      & \textbf{IQL}      & \textbf{DOGE}     & \textbf{TSRL}      & \textbf{Ours}       \\ 
\midrule
Antmaze-u           & 10k (1\%)       & 44.7$\pm$42.1       & 0.7$\pm$1.2         & 0.1$\pm$1.2      & 0.1$\pm$19.4     & 56.3$\pm$24.4    & 65.1$\pm$7.3     & 76.1$\pm$15.6     & \textbf{88.7$\pm$7.7}    \\
Antmaze-u-d         & 10k (1\%)       & 24.1$\pm$22.2       & 16.3$\pm$16.4       & 0.5$\pm$0.1      & 34.6$\pm$18.5    & 41.7$\pm$18.5    & 41.7$\pm$14.2    & 52.2$\pm$22.1     & \textbf{60.9$\pm$16.9}   \\
Antmaze-m-d         & 0.1M (10\%)     & 0.0                 & 0.0                 & 0.0              & 0.0              & 0.0              & 0.0              & 0.0               & \textbf{47.2$\pm$17.3}   \\
Antmaze-m-p         & 0.1M (10\%)     & 0.0                 & 0.0                 & 0.0              & 12.5$\pm$5.4     & 0.0              & 0.0              & 0.0               & \textbf{62.9$\pm$17.8}   \\
Antmaze-l-d         & 0.1M (10\%)     & 0.0                 & 0.0                 & 0.0              & 3.6$\pm$4.1      & 0.0              & 0.0              & 39.8              & \textbf{39.8$\pm$14.1}   \\
Antmaze-l-p         & 0.1M (10\%)     & 0.0                 & 0.0                 & 0.0              & 3.5$\pm$4.1      & 0.0              & 0.0              & 0.0               & \textbf{47.3$\pm$13.1}   \\
\bottomrule
\end{tabular}
\end{adjustbox}
\label{tab:antmaze_results}
\end{table}

\begin{table}[h]
\caption{Positive-valued results on D4RL Franka Kitchen tasks (10k-scale)}
\scriptsize

\begin{adjustbox}{center}
\begin{tabular}{cccccccccc}
\toprule
\textbf{Task}           & \textbf{Size} & \textbf{BC} & \textbf{TD3+BC} & \textbf{MOPO} & \textbf{CQL} & \textbf{IQL} & \textbf{DOGE} & \textbf{TSRL} & \textbf{Ours} \\ 
\midrule
kitchen-mixed-v0       & 10k          & 13.1       & 14.9           & 15.3          & 0.8         & 0.7         & 0.8          & 16.2         & \textbf{18.9$\pm$3.2} \\
kitchen-partial-v0     & 10k          & 4.6        & 3.2            & 0.5           & 0.6         & 0.5         & 3.9          & 5.1          & \textbf{7.9$\pm$0.4} \\
kitchen-complete-v0    & 10k          & 14.2       & 4.5            & 0.3           & 2.1         & 0.4         & 0.2          & 3.8          & \textbf{5.6$\pm$0.3} \\
\bottomrule
\end{tabular}
\end{adjustbox}
\label{tab:kitchen_positive}
\end{table}

\begin{figure}[htbp]
\centering
\subfigure[hopper-medium]{\includegraphics[width=0.3\textwidth]{fig/hopper_m.pdf}}
\subfigure[hopper-medium-replay]{\includegraphics[width=0.3\textwidth]{fig/hopper_mr.pdf}}
\subfigure[hopper-medium-expert]{\includegraphics[width=0.3\textwidth]{fig/hopper_me.pdf}}
\subfigure[hopper-expert]{\includegraphics[width=0.3\textwidth]{fig/hopper_e.pdf}}
\subfigure[walker2d-medium]{\includegraphics[width=0.3\textwidth]{fig/walker2d_m.pdf}}
\subfigure[walker2d-medium-replay]{\includegraphics[width=0.3\textwidth]{fig/walker2d_mr.pdf}}
\subfigure[walker2d-medium-expert]{\includegraphics[width=0.3\textwidth]{fig/walker2d_me.pdf}}
\subfigure[walker2d-expert]{\includegraphics[width=0.3\textwidth]{fig/walker2d_e.pdf}}
\subfigure[halfcheetah-medium]{\includegraphics[width=0.3\textwidth]{fig/halfcheetah_m.pdf}}
\subfigure[halfcheetah-medium-replay]{\includegraphics[width=0.3\textwidth]{fig/halfcheetah_mr.pdf}}
\subfigure[halfcheetah-medium-expert]{\includegraphics[width=0.3\textwidth]{fig/halfcheetah_me.pdf}}
\subfigure[halfcheetah-expert]{\includegraphics[width=0.3\textwidth]{fig/halfcheetah_e.pdf}}

\caption{Locomotion}
\label{fig:pdf_thumbs}
\end{figure}

\begin{figure}[t]
\centering
\subfigure[pen-human]{\includegraphics[width=0.23\textwidth]{fig/pen-human.pdf}}
\subfigure[door-human]{\includegraphics[width=0.23\textwidth]{fig/door-human.pdf}}
\subfigure[hammer-human]{\includegraphics[width=0.23\textwidth]{fig/hammer-human.pdf}}
\subfigure[relocate-human]{\includegraphics[width=0.23\textwidth]{fig/relocate-human.pdf}}
\subfigure[pen-cloned]{\includegraphics[width=0.23\textwidth]{fig/pen-cloned.pdf}}
\subfigure[door-cloned]{\includegraphics[width=0.23\textwidth]{fig/door-cloned.pdf}}
\subfigure[hammer-cloned]{\includegraphics[width=0.23\textwidth]{fig/hammer-cloned.pdf}}
\subfigure[relocate-cloned]{\includegraphics[width=0.23\textwidth]{fig/relocate-cloned.pdf}}
\caption{Adroit}
\label{fig:pdf_adroid}
\end{figure}

\subsection{CL for RL}
$$\max _{\pi}{\mathbb{E}_{s\sim\mathcal{D}_{k}, a\sim\pi(\cdot\mid s)}\left[\widetilde{Q}^{\pi}(s, a)\right]}-{\omega_{1} K\left(\pi,\pi_{k}^{b}\right)}^{}-{\omega_{2} K\left(\pi,\pi^{old}\right)}$$

\begin{theorem}
Suppose that Assumption 1, $(1-\delta_{\pi})\omega_{2}<\omega_{1}<\omega_{2}$, and $\delta_{\pi}>0$ (defined in Eq. (35)) holds. Then, the optimal solution $\pi^{*}$ of the optimization problem
satisfies
$$
J\left(M,\pi^{*}\right) > \max\left\{J(M,\pi^{old}), J\left(M,\pi^{b}\right)\right\}-\epsilon,
$$
with probability greater than $1-2\delta$ and a sufficiently large $\omega_{2}$.
\end{theorem}

\section{Experimental Results}

\subsection{Impletement}
We evaluate our method on the widely recognized offline RL benchmark D4RL\footnote{\url{https://github.com/rail-berkeley/d4rl}} \citep{fu2020d4rl,todorov2012mujoco}, which encompasses two major domains: Gym locomotion control and Maze2D navigation. The Gym domain includes four continuous robotic control tasks ("HalfCheetah", "Hopper", "Walker2d", and "Ant"), each providing four dataset quality levels (expert, medium-expert, medium, and medium-replay). The Maze2D domain requires a 2D agent to navigate to fixed goal positions across three maze sizes ("umaze", "medium", and "large"), featuring both dense and sparse reward variants (as illustrated in Figure~\ref{fig:gym}).

We compare our method against behavior cloning (BC) and state-of-the-art offline RL methods, including model-based approaches like MOPO \citep{yu2020mopo} and model-free methods such as TD3+BC \citep{fujimoto2021minimalist}, CQL \citep{kumar2020conservative}, IQL \citep{iql}, and DOGE \citep{li2022data}. Notably, DOGE demonstrates exceptional out-of-distribution generalization through state-conditioned distance functions. We also include comparisons with TSRL \citep{cheng2023look}, which employs a temporally symmetric dynamics model (TDM) to leverage system dynamics symmetry. This approach enhances offline RL performance on small datasets through reliable latent space data augmentation and OOD sample detection mechanisms enabled by symmetry constraints, significantly improving both data efficiency and generalization capability.
All algorithms are trained for 3-5 times before reporting final normalized performance metrics.

\begin{figure}[h]
	\centering
    \subfigure[Halfcheetah.]{\label{fig:gym-halfcheetah}\includegraphics[width=0.15\textwidth,height=0.14\textwidth]{./fig/gym-halfcheetah.pdf}}
    \hspace{0.02\textwidth}
    \subfigure[Hopper.]{\label{fig:gym-hopper}\includegraphics[width=0.15\textwidth,height=0.14\textwidth]{./fig/gym-hopper.pdf}}
    \hspace{0.02\textwidth}
    \subfigure[Walker2d.]{\label{fig:gym-walker2d}\includegraphics[width=0.15\textwidth,height=0.14\textwidth]{./fig/gym-walker2d.pdf}}
    \hspace{0.02\textwidth}
    \subfigure[Ant.]{\label{fig:gym-ant}\includegraphics[width=0.15\textwidth,height=0.14\textwidth]{./fig/gym-ant.pdf}}
    
	\centering
    \subfigure[Umaze.]{\label{fig:maze-umaze}\includegraphics[width=0.15\textwidth]{./fig/maze2d-umaze.pdf}}
    \hspace{0.01\textwidth}
    \subfigure[Medium.]{\label{fig:maze-medium}\includegraphics[width=0.15\textwidth]{./fig/maze2d-medium.pdf}}
    \hspace{0.01\textwidth}
    \subfigure[Large.]{\label{fig:maze-large}\includegraphics[width=0.15\textwidth]{./fig/maze2d-large.pdf}}
% \caption{Gym maze tasks.} 
% \vspace{-2em}
% \label{fig:gym-maze}
\caption{Gym locomotion and Maze2D tasks.} 
% \vspace{-2em}
\label{fig:gym}
\end{figure}

\subsection{Evaluation on D4RL locomotion Gym Tasks}
We evaluate each method on the D4RL locomotion Gym tasks, which include three distinct environments: half-cheetah, hopper, and walker2d. For each environment, we analyze six datasets generated by different policies. These datasets consist of transitions collected by a random policy with uniform action sampling, an expert policy with fully trained performance, a medium policy achieving approximately one-third of the expert's performance, a medium-expert mixture combining medium and expert trajectories, a medium-replay buffer containing data from a policy trained to medium performance, and a full-replay buffer comprising the expert's final training data.  

All datasets except medium-replay contain one million transitions. The medium-replay dataset differs in size as it represents the replay buffer of a policy trained to medium performance rather than a fixed collection. This comprehensive evaluation framework allows us to thoroughly assess the robustness and generalization capabilities of each method across diverse data distributions and performance levels.

\newpage
\newpage
% \section*{References}

% References follow the acknowledgments in the camera-ready paper. Use unnumbered first-level heading for
% the references. Any choice of citation style is acceptable as long as you are
% consistent. It is permissible to reduce the font size to \verb+small+ (9 point)
% when listing the references.
% Note that the Reference section does not count towards the page limit.
% \medskip

%%%%%%%%%%%%%%%%%%%%%%%%%%%%%%%%%%%%%%%%%%%%%%%%%%%%%%%%%%%%
\newpage
\appendix

\section{Sample error}
Under NTK assumption, we have
$$\hat Q(x) - \hat Q(x_{in})\leq \beta(\mathcal{D})\left(\sqrt{C_X |x-x_{in}|}+2|x-x_{in}|\right)=\beta(\mathcal{D})g(x,x_{in})$$
with $x=(\bs,\ba)$ and $x_{\rm in} \in \mathcal{D}$.
We assume reward is bounded, \ie, $r(\bs,\ba)\in[-R_{\rm max},R_{\rm max}]$.
The difference between the empirical Bellman operator and the actual Bellman operator can be bounded:
\begin{align*}
    &\left\vert\hat{\bellman}^\policy \hat{Q}^k (x) - {\bellman}^\policy \hat{Q}^k(x) \right\vert \\
    =& \left\vert\left(r - r(\bs, \ba)\right) + \gamma \int_{\bs'} \left(\hat{\transitions}(\bs'|\bs, \ba) - \transitions(\bs'|\bs,\ba)\right) \E_{\policy(\ba'|\bs')}\left[\hat{Q}^k(\bs' , \ba')\right]d\bs'\right\vert\\
    \leq& \left\vert r - r(\bs, \ba)\right\vert + \gamma \left\vert \int_{\bs'} \left(\hat{\transitions}(\bs'|\bs, \ba) - \transitions(\bs'|\bs,\ba)\right) \E_{\policy(\ba'|\bs')}\left[\hat{Q}^k(\bs' , \ba')\right]d\bs'\right\vert\\
    \mathop{=}^{(a)}& \left\vert r - r(\bs, \ba)\right\vert
    + \min_{\bs_D,\ba_D \in \mathcal{D}}\gamma \left\vert \int_{\bs'} \left(\hat{\transitions}(\bs'|\bs, \ba) - \transitions(\bs'|\bs,\ba)\right) \left(\E_{\policy(\ba'|\bs')}\left[\hat{Q}^k(\bs' , \ba')\right]
     -\E_{\policy(\ba'|\bs')}\left[\hat{Q}^k(\bs_D , \ba_D)\right]\right)d\bs'\right\vert\\
    \mathop{\leq}^{}& \left\vert r - r(\bs, \ba)\right\vert
    + \gamma \left\vert \int_{\bs'} \hat{\transitions}(\bs'|\bs, \ba)\int_{\ba'} \policy(\ba'|\bs') \left(\hat{Q}^k(\bs' , \ba')-\hat{Q}^k(\bs_{t+1} , \ba_{t+1})\right)d\ba'd\bs'\right\vert\\
    & + \gamma \left\vert \int_{\bs'} {\transitions}(\bs'|\bs, \ba)\int_{\ba'} \policy(\ba'|\bs') \left(\hat{Q}^k(\bs_{t+1} , \ba_{t+1})-\hat{Q}^k(\bs' , \ba')\right)d\ba'd\bs'\right\vert\\
    \mathop{\leq}^{(b)}& 2R_{max}
    + \gamma \beta(\mathcal{D})\left(\sqrt{C_X |\mathcal{A}|}+2|\mathcal{A}|\right)
    + \gamma \beta(\mathcal{D}) \left\vert \int_{\bs'} {\transitions}(\bs'|\bs, \ba)\int_{\ba'} \left(\hat{Q}^k(\bs_{t+1} , \ba_{t+1})-\hat{Q}^k(\bs' , \ba')\right)d\ba'd\bs'\right\vert\\
    \mathop{\leq}^{}& 2R_{max}
    + \gamma \beta(\mathcal{D})\left(\sqrt{C_X |\mathcal{A}|}+2|\mathcal{A}|\right)
    + \gamma \beta(\mathcal{D}) \mathbb{E}_{x'=(s',a')\sim T(s'|x)\pi(a'|s')} g(x',x_{t+1})
    =\Delta(x,\mathcal{D})
    % + 2\gamma c_1 G(|x'-x_D|)\\
    % \leq& C_{r, \delta} + 2\gamma \min\left\{ c_1 G(|x'-x_D|), \frac{C_{T, \delta} R_{\max}}{(1 - \gamma)\sqrt{\max\{1,|\mathcal{D}_{s,a}|\}}}\right\} 
    % ~~\text{(since limited data, $\sqrt{\max\{1,|\mathcal{D}_{s,a}|\}}\approx 1$)}\\
    % =& C_{r, \delta} + 2\gamma \beta(\mathcal{D}) g(x',\mathcal{D})~~\text{(The small $\mathcal{D}$ leads to a large, non-negligible $\frac{C_{T, \delta} R_{\max}}{(1 - \gamma)\sqrt{\max\{1,|\mathcal{D}_{s,a}|\}}}$)}\\
    % =& C_{r, \delta}
    % + 2\gamma C_{\beta} (C_x\sqrt{|x'-x_D|)}+2|x'-x_D|)
    % % =& C_{r, \delta} + 2\gamma C_{\beta} (C_x\sqrt{2(|\mathcal{S}|+|\mathcal{A}|)}+4|\mathcal{S}|+4|\mathcal{A}|)
    % = \Delta_{a}.
\end{align*}
% with $x=(\bs,\ba)$.
% where 
(a) holds because $(\bs_D,\ba_D) \in \mathcal{D}$ is independent with $(\bs' , \ba')$, which implies 
\begin{align}
    &\int_{\bs'} \left(\hat{\transitions}(\bs'|\bs, \ba) - \transitions(\bs'|\bs,\ba)\right) \E_{\policy(\ba'|\bs')}\left[\hat{Q}^k(\bs_D , \ba_D)\right] d\bs'\\
=&\left(\int_{\bs'} \hat{\transitions}(\bs'|\bs, \ba)d\bs' - \int_{\bs'}\transitions(\bs'|\bs,\ba)d\bs'\right) \E_{\policy(\ba'|\bs')}\left[\hat{Q}^k(\bs_D , \ba_D)\right]\\
=&(1-1)\E_{\policy(\ba'|\bs')}\left[\hat{Q}^k(\bs_D , \ba_D)\right]= 0.
\end{align}
% $$$$
% where 
(b) holds if $(\bs_{t+1},\ba_{t+1})\in\mathcal{D}$, we have
\begin{align}
&\min_{\bs_D,\ba_D \in \mathcal{D}}\gamma \left\vert \int_{\bs'} \hat{\transitions}(\bs'|\bs, \ba)\int_{\ba'} \policy(\ba'|\bs') \left(\hat{Q}^k(\bs' , \ba')-\hat{Q}^k(\bs_D , \ba_D)\right)d\ba'd\bs'\right\vert\\
\leq& \gamma \left\vert \int_{\ba'} \policy(\ba'|\bs_{t+1}) \left(\hat{Q}^k(\bs_{t+1} , \ba')-\hat{Q}^k(\bs_{t+1},\ba_{t+1})\right)d\ba'\right\vert\\
\leq& \gamma \left\vert \int_{\ba'} \policy(\ba'|\bs_{t+1}) d\ba'\right\vert
\max_{\ba'}\left\vert \left(\hat{Q}^k(\bs_{t+1} , \ba')-\hat{Q}^k(\bs_{t+1},\ba_{t+1})\right)\right\vert\\
\leq& \gamma \beta(\mathcal{D})\left(\sqrt{C_X |\mathcal{A}|}+2|\mathcal{A}| \right)
\end{align}

% Thus, we have

\newpage
For any $x \in \mathcal{D}_i$ and $\mathcal{D} = \cup_{i\in K}\mathcal{D}_i $, we have
\begin{align}
    &\Delta(x,\mathcal{D}) - \Delta(x,\mathcal{D}_i)\\
    = &\gamma \left(\beta(\mathcal{D})-\beta(\mathcal{D}_i)\right)\left(\sqrt{C_X |\mathcal{A}|}+2|\mathcal{A}|+\mathbb{E}_{x'=(s',a')\sim T(s'|x)\pi(a'|s')} g(x',x_{t+1})\right)\\
    \geq &\gamma \left(\beta(\mathcal{D})-\beta(\mathcal{D}_i)\right)\left(\sqrt{C_X |\mathcal{A}|}+2|\mathcal{A}|\right) \geq 0.
\end{align}
according to Propositions \ref{pro:beta} and \ref{pro:D-i}.
Assume that a set of Q-value functions $Q_i$ is trained on each $D_i$. For any input $x$, we can always find at least one $Q_i$ whose sampling error is smaller than the sampling error of $Q$ training-based $D$.

The principles for partitioning datasets are as follows:

1. The entire dataset $\mathcal{D}$ is the union of all subsets $\mathcal{D}_i$, formally expressed as $\mathcal{D} = \bigcup_{i\in K}\mathcal{D}_i$, where $K$ is an index set. This ensures that all data points are accounted for within the partitioned subsets.

2. Given a data point $(\mathbf{s}_{t}, \mathbf{a}_{t})$ belonging to a particular subset $\mathcal{D}_i$, it is highly desirable that the subsequent data point $(\mathbf{s}_{t + 1}, \mathbf{a}_{t + 1})$ also belongs to the same subset $\mathcal{D}_i$. This principle helps maintain the contextual integrity and temporal coherence of the data within each subset.

3. Overlapping between datasets is permitted. That is, it is acceptable for some data points to be shared among multiple subsets $\mathcal{D}_i$. This flexibility can be beneficial in certain scenarios where data points may have relevance across different partitions.

\section{Data Splitting}
\begin{proposition}
\label{pro:beta}
    % $\beta(\mathcal{D})$ 是一个关于数据集$\mathcal{D}$的单调非减的子模函数
    The set function \(\beta: 2^\mathcal{X} \to \mathbb{R}\) defined over a dataset \(\mathcal{D} \subseteq \mathcal{X}\) is
    \begin{itemize}
        \item \textbf{Monotone non-decreasing}: For any \(\mathcal{D}_1 \subseteq \mathcal{D}_2 \subseteq \mathcal{X}\), we have \[ \beta(\mathcal{D}_1) \leq \beta(\mathcal{D}_2). \]
        \item \textbf{Submodular}: For any \(\mathcal{D}_1 \subseteq \mathcal{D}_2 \subseteq \mathcal{X}\) and \(d \in \mathcal{X} \setminus \mathcal{D}_2\), we have
        \[ \beta(\mathcal{D}_1 \cup \{d\}) - \beta(\mathcal{D}_1) \geq \beta(\mathcal{D}_2 \cup \{d\}) - \beta(\mathcal{D}_2). \]
        \item \textbf{upper bound}: $\beta(\mathcal{D})\leq C_{\beta},  \forall \mathcal{D}$.  \cite{li2022data}
    \end{itemize}
    according to \ref{app:beta} and references \cite{wiki_submodular_set_function,fujishige2005submodular}
\end{proposition}
Proposition \ref{pro:beta} implies that $\beta(\mathcal{D})$ is a submodular non-decreasing set function, which explain why sample error becomes larger with $\mathcal{D}$ larger samples.

\begin{proposition}
\label{pro:g}
    A set function $g: 2^\mathcal{X} \to \mathbb{R}$ is \textbf{supermodular} if for any subsets $\mathcal{D}_1, \mathcal{D}_2 \subseteq \mathcal{X}$, it satisfies: 
    $$ g(x', \mathcal{D}_1 \cup \mathcal{D}_2) + g(x', \mathcal{D}_1 \cap \mathcal{D}_2) \geq g(x', \mathcal{D}_1) + g(x', \mathcal{D}_2). $$ 
    For any \(\mathcal{D}_1 \subseteq \mathcal{D}_2 \subseteq \mathcal{X}\), we have
    $$ g(x', \mathcal{D}_1) \geq g(x', \mathcal{D}_2). $$ 
    Additionally, we have the lower bound $g(x', \mathcal{D})\geq 0, \forall \mathcal{D}$ and $\lim_{|\mathcal{D}| \to |\mathcal{X}|} g(x',\mathcal{D}) = 0$.
    % If the inequality holds strictly when $\mathcal{D}_1$ and $\mathcal{D}_2$ are incomparable (i.e., neither $\mathcal{D}_1 \subseteq \mathcal{D}_2$ nor $\mathcal{D}_2 \subseteq \mathcal{D}_1$), $G$ is called strictly supermodular.
\end{proposition}
Proposition \ref{pro:g} establishes that $g(x',\mathcal{D})$ is a supermodular non-increasing set function. This property explains the asymptotic convergence of the sample error to zero as the dataset $\mathcal{D}$ becomes sufficiently large.

\begin{proposition}
\label{pro:next_sa}
    For limited data, \(\hat{T}\) becomes deterministic \ie $\hat{T}(s_{t+1}|s_t,a_t) = 1$. 
    If $(\bs_t,\ba_t)\in \mathcal{D}$ and $(\bs_{t+1},\ba_{t+1})\in \mathcal{D}$, we derive 
    % $$\beta(\mathcal{D}) g(x',\mathcal{D}) \leq C_{\beta} (C_x\sqrt{4|\mathcal{A}|+2d_{\rm{max}}}+8|\mathcal{A}|+4d_{\rm{max}})$$
    $$\Delta_{a} = C_{r, \delta} + \gamma C_{\beta} (C_x\sqrt{|x'-x_D|)}+2|x'-x_D|+C_x\sqrt{|\mathcal{A}|}+2|\mathcal{A}|)$$
where $d_{\rm{max}}$ denotes the maximal distance from $\bs$ to $\bs'$, $d_{\rm{max}}\leq|\mathcal{S}|$.
\end{proposition}
Proposition \ref{pro:next_sa} shows that if the next state and next action turple $x'=(s',a')\in\mathcal{S}$, we obtain $\Delta_{a}$ admits a tighter lower bound.

\begin{proposition}
\label{pro:D-i}
    For any $x$ and $\mathcal{D} = \cup_{i\in K}\mathcal{D}_i $, we have
    \begin{align}
        \min_i\{\beta(\mathcal{D}_i)g(x, \mathcal{D}_i)\}
        \leq \beta(\mathcal{D}) g(x, \mathcal{D})
    \end{align}
\end{proposition}
\begin{proof}
    For any $x$ and $\mathcal{D} = \cup_{i\in K}\mathcal{D}_i $, we have
    \begin{align}
        g(x, \mathcal{D})=\min_i\{g(x, \mathcal{D}_i)\},\\
        \beta(\mathcal{D})\geq \beta(\mathcal{D}_i),~~\forall \mathcal{D}_i,
    \end{align}
    according to Proposition \ref{pro:beta} and Proposition \ref{pro:g}.
    % where $\mathcal{D} = \cup_{i\in K}\mathcal{D}_i $
    Thus, we obtain the following
    \begin{align}
        \min_i\{\beta(\mathcal{D}_i)g(x, \mathcal{D}_i)\}
        \leq \min_i\{\beta(\mathcal{D})g(x, \mathcal{D}_i)\}
        = \beta(\mathcal{D}) \min_i\{g(x, \mathcal{D}_i)\}
        = \beta(\mathcal{D}) g(x, \mathcal{D})
    \end{align}
\end{proof}
Proposition \ref{pro:D-i} demonstrates that the dataset partitioning method can effectively reduce sampling errors.

\section{Monotonic Non-Decreasing Property of $\beta(n)$ }
\subsection{Notation Definition and Initial Setup}
Let's start by clearly defining our notations. Consider the original training data set, denoted as 
$$\{x_1, x_2, \ldots, x_n\}.$$ 
The space spanned by the corresponding feature maps of this original training data is 
$$W = \text{span}(\phi(x_1), \phi(x_2), \ldots, \phi(x_n)).$$

In the Reproducing Kernel Hilbert Space (RKHS), we represent the function $f_{\text{NTK}}$ in terms of its coordinates $\beta_{\text{NTK}}$. This $\beta_{\text{NTK}}$ can be decomposed into two components. We write $\beta_{\text{NTK}}=\beta_0 + \beta_1$, where $\beta_0$ represents the component of $f_{\text{NTK}}$ that lies within the space $W$. On the other hand, $\beta_1$ is the component that exists in the orthogonal complement of $W$, denoted as $W^{\perp}$.

Now, let's consider the situation when we expand our training data set. We add new training data points, which are given by $\{x_{n + 1}, x_{n+2}, \ldots, x_{n + m}\}$. With the inclusion of these new data points, the space spanned by the feature maps changes. The new space, denoted as $W'$, is defined as 
$$W'=\text{span}(\phi(x_1), \phi(x_2), \ldots, \phi(x_{n+m})).$$

Correspondingly, in the RKHS, the coordinate representation of $f_{\text{NTK}}$ also undergoes a change. We now have $\beta_{\text{NTK}}'=\beta_0'+\beta_1'$. Here, $\beta_0'$ is the component of $f_{\text{NTK}}$ within the new space $W'$, while $\beta_1'$ is the component in the orthogonal complement of $W'$, which is $W'^{\perp}$.

\subsection{Properties Based on Kernel Regression}
For the original training data set, we have a specific relationship based on kernel regression. We know that $\phi(x_i)^{\top}\beta_{\text{NTK}} = y_i$ for each $i$ ranging from $1$ to $n$. Here, $y_i$ represents the corresponding label for the training data point $x_i$.
The component $\beta_0$ is uniquely determined by the kernel regression solution with respect to the Neural Tangent Kernel (NTK). The function $f_{\text{NTK}}(x)$ can be expressed as  
$$f_{\text{NTK}}(x)= (\langle\phi(x),\phi(x_1)\rangle, \ldots, \langle\phi(x),\phi(x_n)\rangle)\cdot\text{NTK}_{\text{train}}^{-1}Y.$$
In this expression, $\text{NTK}_{\text{train}}$ is the $n\times n$ kernel matrix of the original training data. The term $\langle\phi(x),\phi(x_i)\rangle$ represents the kernel between the test data $x$ and the training data $x_i$. $Y$ is the vector containing all the training labels for the original data set.

When we incorporate the new training data points, the situation evolves. For the combined data set with indices $i$ from $1$ to $n + m$, we have $\phi(x_i)^{\top}\beta_{\text{NTK}}' = y_i$. The new kernel regression solution for the function $f_{\text{NTK}}'(x)$ is given by 
$$f_{\text{NTK}}'(x)= (\langle\phi(x),\phi(x_1)\rangle, \ldots, \langle\phi(x),\phi(x_{n + m})\rangle)\cdot\text{NTK}_{\text{train}}'^{-1}Y'.$$
Here, $\text{NTK}_{\text{train}}'$ is the $(n + m)\times(n + m)$ kernel matrix of the expanded training data set, and $Y'$ is the updated label vector that includes the labels for the new data points as well.

\subsection{Analyzing the Norm Change of $\beta$}
\label{app:beta}
To understand how the norm of $\beta$ changes, we need to consider the properties of orthogonal decomposition. Since $W$ is a subspace of $W'$, for any vector $v$, its orthogonal decomposition in $W'$ is $\mu = v_0 + v_1$, where $v_0\in W'$ and $v_1\in W'^{\perp}$. In the space $W$, the orthogonal decomposition of the same vector $v$ is $\mu = v_{00}+v_{01}$, with $v_{00}\in W$ and $v_{01}\in W^{\perp}$.

We know from the properties of orthogonal decomposition that $\|v\|_2^2=\|v_0\|_2^2+\|v_1\|_2^2$ and $\|v\|_2^2=\|v_{00}\|_2^2+\|v_{01}\|_2^2$. Moreover, we have the relationship $\|v_0\|_2\geq\|v_{00}\|_2$.

When we look at $\beta_{\text{NTK}}$ and $\beta_{\text{NTK}}'$, we note that $\beta_{\text{NTK}}$ is designed to satisfy the fitting condition for the original training data. That is, it is the solution to the optimization problem $\min_{\beta}\|\beta\|_2$ subject to the constraints $\phi(x_i)^{\top}\beta = y_i$ for $i$ from $1$ to $n$.

On the other hand, $\beta_{\text{NTK}}'$ is the solution to a similar optimization problem, but for the expanded training data set. It solves $\min_{\beta}\|\beta\|_2$ subject to $\phi(x_i)^{\top}\beta = y_i$ for $i$ from $1$ to $n + m$.

The new optimization problem with the additional training data has a more restricted feasible region. The feasible region for the new problem is a subset of the original feasible region because it now has to satisfy the fitting conditions for more data points. According to the principles of optimization theory, when the feasible region becomes more restricted in this way, the minimum value of the objective function (in this case, the norm of $\beta$) will not decrease. Hence, we can conclude that $\|\beta_{\text{NTK}}'\|_{\infty}\geq\|\beta_{\text{NTK}}\|_{\infty}$.

The infinitynorm $\|\cdot\|_{\infty}$ of a vector is defined as the value of its largestabsolutevalue element. Since $\beta_{\text{NTK}}'$ and $\beta_{\text{NTK}}$ are constructed based on kernel regression to fit the training data, the addition of new data points restricts the solution space further. This restriction ensures that the infinitynorm of $\beta$ either increases or at least remains the same. 

In conclusion, when we add some training data to our dataset, the infinity-norm of $\beta$ will either increase or, at the very least, not decrease. 

\section{Others}
\subsection{MoE+RL}
$$
\mathcal{L}_{freq} = (\mu - w)(\mu - w)^T, w = [w_1, \cdots, w_{K}],
$$

$v$ is a one-hot code vector $\mu = [\mu_1, \mu_2, \cdots, \mu_K]$  with
$$
\mu_j = 
\begin{cases}
1, & \text{if } j = \arg\max_i Q_{i}(\bs, \ba); \\
0, & \text{otherwise}.
\end{cases}
$$

\begin{align}
\pi_{moe}(\ba|\bs)=\sum_{i = 1}^{K}w_{i}(\bs)\pi_{i}(\ba|\bs), ~~~~
\text{s.t. } \sum_{i = 1}^{K}w_{i}=1, w_{i}>0, 
\end{align}

For the gating operation, the outputs of the weight operation are the weights of each action from different policies. With those weights, the gating operation uses the weighted action as the final output action
\begin{align}
\ba=\sum_{i = 1}^{K}w_{i}(\bs)\ba_i, ~~~~
\text{s.t. } a_i\sim  \pi_{i}(\ba|\bs), 
\end{align}
according to \citep{peng2019mcp}.

\subsubsection{CL}
\[
\pi_{t+i} \leftarrow \arg\max_{\pi_{t+i}} \mathbb{E}_{s \sim D_{i}, a \sim \pi_{t+i}(\cdot | s)}[\widehat{Q}_{t+i}^\pi(s, a)] - \theta_1 D(\pi_{t+i}, \pi_{\beta, i}) - \theta_2 D(\pi_{t+i}, \pi_{t+i-1}),
\]
